# Supplementary material for: The Label Complexity of Useful Class-Conditional Prediction Sets under Distribution Shift
Source: arXiv:2607.18088 source file (2026-10-05)
Supplement: Supplementary file 1 [file supplement.tex]

\pdfoutput=1
\documentclass[twoside]{article}

\usepackage[preprint]{aistats2026}

\usepackage{amsmath,amssymb,amsthm}
\usepackage{booktabs}
\usepackage{graphicx}
\graphicspath{{figures/}{./}}
\usepackage{xcolor}
\usepackage{hyperref}
\usepackage[round]{natbib}
\usepackage{enumitem}

\hypersetup{colorlinks=true,linkcolor=blue,citecolor=blue,urlcolor=blue}
\emergencystretch=3em

\theoremstyle{plain}

\newtheorem{proposition}{Proposition}
\newtheorem{lemma}{Lemma}
\newtheorem{corollary}{Corollary}
\theoremstyle{definition}

\theoremstyle{remark}
\newtheorem{remark}{Remark}

\newcommand{\SPD}{\mathrm{SPD}}
\newcommand{\LE}{\mathrm{LE}}

\newcommand{\dg}{d_{g}}
\newcommand{\dLE}{d_{\LE}}
\newcommand{\Mc}{M_{c}}
\newcommand{\R}{\mathbb{R}}

\newcommand{\Log}{\mathrm{Log}}
\newcommand{\Exp}{\mathrm{Exp}}
\newcommand{\GL}{\mathrm{GL}}
\newcommand{\vech}{\mathrm{vech}}
\newcommand{\sig}{s}

\begin{document}

\runningtitle{Supplementary Material: Label Complexity of Class Conditional Coverage}

\onecolumn
\aistatstitle{Supplementary Material: The Label Complexity of Class Conditional Coverage\\ under Distribution Shift}

\paragraph{Abbreviations.}
SPD = symmetric positive definite; ST-GCN / CTR-GCN = the spatial temporal and channel wise
topology refined graph convolutional network backbones; LAC / APS / RAPS = the least ambiguous
set valued classifier, adaptive prediction sets, and regularized APS nonconformity scores;
OOD = out of distribution; AUROC = area under the ROC curve; CRC = conformal risk control;
PPI = prediction powered inference; CP = conformal prediction; LE = log Euclidean;
xsub / xview = the NTU cross subject and cross view evaluation splits.

\section{Construction and proof of the impossibility proposition}
\label{supp:impossible_proof}

The main paper states the impossibility proposition (no valid \emph{and} efficient label free
per class coverage under joint shift); its construction and proof follow.

\medskip
\noindent\emph{Construction.} By the score separation assumption of the proposition, fix
disjoint regions $B,A$ with
\begin{align*}
P_T(B)&>0, & P_T(A)&=m>0, \\
\inf_{x\in A}s(x,c)&\ge q_B+\delta,
\end{align*}
where $q_B$ is the $(1{-}\alpha)$-quantile of $s(X,c)$ on the class-$c$ base population in $B$.
Both laws place class $c$ on $B$ with mass $\mu_c>0$ chosen so that
\[
\varepsilon:=\frac{m}{m+\mu_c}>\alpha.
\]
$P_T'$ assigns the $A$-mass to $Y{=}c$, whereas $P_T$ assigns it to some $c'\ne c$. Thus,
\begin{align*}
q_c^\star(P_T')&\ge q_B+\delta, \\
q_c^\star(P_T)&=q_B.
\end{align*}
Both joints share $P_T(X)$ and are consistent with $P_S$, since label free observables place no
restriction on $P_T(Y\mid X)$; class $c$ has positive mass under both. Validity under $P_T'$ forces
\[
\Pr[c\in\hat C(X)\mid X\in A]\ge\frac{\varepsilon-\alpha}{\varepsilon}.
\]
Under $P_T$ these inclusions are spurious, and deleting them preserves validity on $P_T$ (class $c$
has no $A$-mass there) while cutting expected size by at least
\[
\beta=\frac{m(\varepsilon-\alpha)}{\varepsilon}.
\]
$\qed$

\medskip
\noindent\emph{Relation to classical impossibility results.} Unlike the classical impossibility of
distribution free \emph{conditional} coverage \citep{vovk2012conditional,leiwasserman2014,barber2021limits},
which stems from the nonatomicity of $X$ within a single unknown i.i.d.\ law (attainable by
Mondrian CP given labels), our obstruction is an identification failure \emph{across} laws:
$(P_S,P_T(X))$ does not identify the target class conditional score law under unrestricted
$P_T(Y\mid X)$, at the same set size inflation price that worst case robust conformal methods pay
by design \citep{cauchois2024robust}. Group conditional generalizations that unify class and
covariate conditional coverage \citep{bairaktari2025kandinsky} enrich the covering family under a
\emph{fixed, known} law and assume a known source to target density ratio, so they sidestep the
label free identification failure our result isolates; they do not resolve it.

\begin{corollary}[When label free recovery is possible]
\label{cor:impossible}
Valid \emph{and} efficient target per class coverage label free requires an identifying restriction
on $P_T(Y\mid X)$: covariate shift ($p(y\mid x)$ invariant, so class conditional weighted CP with the
covariate ratio is valid given $P_T(X)\ll P_S(X)$, approximate with estimated weights,
\citealp{tibshirani2019}), or label shift ($p(x\mid y)$ invariant with $\pi_c^T>0$, so source
Mondrian applies, \citealp{podkopaev2021labelshift}). Under a joint shift satisfying \emph{neither}
restriction, as in the main paper's cross sensor NTU$\to$N-UCLA shift, where source thresholds
transfer neither marginally nor per class, any method valid over the identified set must calibrate
to its worst case and hence overcovers on non extremal laws (empirically, weighted CP here). Any
method matching oracle efficiency on one consistent law undercovers on another instead (the
geometric candidate's failure mode); none matches the target label oracle uniformly. The strongest
honest guarantee is then assumption conditional, with a slack that is not point identified from
$(P_S,P_T(X))$ (only worst case one sided bounds are available label free). This is the theoretical
boundary that the main paper's severity spectrum experiments trace empirically.
\end{corollary}

\section{Proof of the label complexity theorem}
\label{supp:labelcomplexity_proof}

We prove the label complexity theorem (main paper, Theorem~1) for the single validity notion stated
there. For a
target law $P$, define
\[
\mathcal V(P)=
\left\{F_c^T(\hat q_c)\ge1-\alpha\ \text{for every }c\right\},
\qquad
\mathcal E_\varepsilon(P)=
\left\{\max_c|\hat q_c-q_c^\star|\le\varepsilon\right\}.
\]
Both are events over the labeled audit and any internal randomization. Every upper and lower bound
below concerns $P_{\mathcal A}\{\mathcal V(P)\cap\mathcal E_\varepsilon(P)\}$ for a classwise
threshold predictor.

\subsection*{(a) Simultaneous PAC validity}
Condition on the audit counts $(m_c)_c$. The class-$c$ scores
$S_{c,1},\ldots,S_{c,m_c}$ are i.i.d.\ from $F_c^T$. For $m_c>0$, write
\[
\widehat F_c(t)=\frac1{m_c}\sum_{i=1}^{m_c}\mathbf 1\{S_{c,i}\le t\},
\qquad
e_c=\sqrt{\frac{\log(2K/\delta)}{2m_c}}.
\]
The Dvoretzky-Kiefer-Wolfowitz inequality gives
\[
P_{\mathcal A}\left\{\sup_t|\widehat F_c(t)-F_c^T(t)|>e_c\right\}
\le 2e^{-2m_ce_c^2}=\frac{\delta}{K}.
\]
A union bound shows that the events
\[
\mathcal D_c=\left\{\sup_t|\widehat F_c(t)-F_c^T(t)|\le e_c\right\}
\]
hold simultaneously with probability at least $1-\delta$.

If $m_c=0$, PAC Audit Mondrian sets $\hat q_c=+\infty$, so
$F_c^T(\hat q_c)=1$. If $m_c>0$ and $\gamma_c=1-\alpha+e_c\ge1$, it makes the same choice.
Suppose $m_c>0$ and $\gamma_c<1$. The selected order statistic has
$k_c=\lceil m_c\gamma_c\rceil$, hence
\[
\widehat F_c(\hat q_c)=\frac{k_c}{m_c}\ge\gamma_c.
\]
On $\mathcal D_c$,
\[
F_c^T(\hat q_c)
\ge\widehat F_c(\hat q_c)-e_c
\ge\gamma_c-e_c
=1-\alpha.
\]
This proves $P_{\mathcal A}\{\mathcal V(P)\}\ge1-\delta$ without a restriction on
$P_T(Y\mid X)$.

For comparison, the ordinary uninflated conformal threshold uses the
$\lceil(m_c+1)(1-\alpha)\rceil$-th audit score, with $+\infty$ when that index exceeds $m_c$.
The index is finite exactly when
\[
\lceil(m_c+1)(1-\alpha)\rceil\le m_c,
\]
which is equivalent to $m_c\ge\lceil1/\alpha\rceil-1$. Below this threshold the $+\infty$
convention remains valid because class $c$ is always included. Thus $m_c=9$ at $\alpha=0.1$ is the
first finite ordinary conformal threshold. It is a non-vacuity threshold and is unrelated to the
existence of a validity guarantee. PAC Audit Mondrian has its own finite-threshold condition
$e_c<\alpha$. \hfill$\square$

\subsection*{(b) Sufficiency for quantile recovery}
Assume $F_c^T$ is continuous and has density at least $f_{0c}>0$ on
$[q_c^\star,q_c^\star+r_c]$. Fix a class for which $\gamma_c<1$. Since
$k_c/m_c<\gamma_c+1/m_c$, the DKW event gives
\begin{align}
F_c^T(\hat q_c)
&\le \widehat F_c(\hat q_c)+e_c \notag\\
&< \gamma_c+\frac1{m_c}+e_c \notag\\
&=1-\alpha+2e_c+\frac1{m_c}.
\label{eq:pac_mondrian_cdf_upper}
\end{align}
Part (a) gives the lower inequality
\[
F_c^T(\hat q_c)\ge1-\alpha=F_c^T(q_c^\star).
\]
The density lower bound makes $F_c^T$ strictly increasing on the stated interval. It follows first
that $\hat q_c\ge q_c^\star$. If
\[
B_c=\frac{2e_c+m_c^{-1}}{f_{0c}}\le r_c,
\]
then $\hat q_c$ cannot exceed $q_c^\star+B_c$: otherwise integration of the density lower bound
would give
\[
F_c^T(\hat q_c)-F_c^T(q_c^\star)
>f_{0c}B_c
=2e_c+\frac1{m_c},
\]
contradicting \eqref{eq:pac_mondrian_cdf_upper}. Therefore, simultaneously on
$\bigcap_c\mathcal D_c$,
\[
0\le\hat q_c-q_c^\star
\le
\frac{1}{f_{0c}}\left\{
2\sqrt{\frac{\log(2K/\delta)}{2m_c}}+\frac1{m_c}\right\}.
\]
This proves the claimed probability $1-\delta$ for validity and quantile recovery under the one
procedure.

Here is one explicit sufficient sample size. Put $h_c=\min\{\varepsilon,r_c\}$ and
$\ell=\log(2K/\delta)$. The three conditions
\[
m_c\ge
\max\left\{
\frac{8\ell}{f_{0c}^2h_c^2},
\frac{2}{f_{0c}h_c},
\frac{\ell}{2\alpha^2}
\right\}
\]
imply $2e_c\le f_{0c}h_c/2$, $m_c^{-1}\le f_{0c}h_c/2$, and $e_c\le\alpha$.
With strict inequalities, the selected threshold is finite and
$0\le\hat q_c-q_c^\star\le h_c\le\varepsilon$. This yields
$m_c=O(\varepsilon^{-2}\log(K/\delta))$ when $\alpha,f_{0c},r_c$ are fixed. \hfill$\square$

\subsection*{Expected set size corollary}
For every deterministic threshold vector $q$,
\[
\mathbb E_{P_T}|\hat C_q(X)|
=\sum_{c=1}^K P_T\{s(X,c)\le q_c\}
=\sum_{c=1}^K G_c(q_c).
\]
On the event proved in part (b), both $q_c^\star$ and $\hat q_c$ lie in the interval on which
$G_c$ is $L_c$-Lipschitz, and $\hat q_c\ge q_c^\star$. Consequently,
\begin{align*}
0
&\le
\mathbb E_{P_T}|\hat C_{\hat q}(X)|
-\sum_{c=1}^K G_c(q_c^\star) \\
&=\sum_{c=1}^K\{G_c(\hat q_c)-G_c(q_c^\star)\} \\
&\le\sum_{c=1}^K L_c(\hat q_c-q_c^\star) \\
&\le
\sum_{c=1}^K\frac{L_c}{f_{0c}}
\left\{
2\sqrt{\frac{\log(2K/\delta)}{2m_c}}+\frac1{m_c}
\right\}.
\end{align*}
The constants $L_c$ are part of the conclusion. No lower bound for this unnormalized total is
claimed. \hfill$\square$

\subsection*{Lower bounds for the label complexity theorem}
The formal lower-bound statements retain the existing labels used elsewhere in the paper.

\begin{lemma}[Necessity, for a suitable shift instance]
\label{supp:lem:necessity}
Fix $\alpha\in(0,1)$. There are a score, a source law, a target covariate law, and constants
$c_0,\varepsilon_0>0$ such that, for every $0<\varepsilon\le\varepsilon_0$, two target laws share
the same $(P_S,P_T(X))$ and satisfy the following property. Every classwise threshold procedure
using the full source law, an unbounded unlabeled target pool, and
$m\le c_0\varepsilon^{-2}$ labeled target pairs has
\[
\max_{P\in\{P_+,P_-\}}
P_{\mathcal A,P}\{\mathcal V(P)^c\cup\mathcal E_\varepsilon(P)^c\}
\ge\frac14.
\]
\end{lemma}

\begin{lemma}[The $\log K$ term is necessary]
\label{supp:lem:logK}
There is an instance with $K$ foreground classes and one background class. Let $n_c$ be a fixed
quota of labeled target pairs drawn from observed region $c$. If a classwise threshold procedure
satisfies
\[
\inf_a P_{\mathcal A,P_a}
\{\mathcal V(P_a)\cap\mathcal E_\varepsilon(P_a)\}\ge\frac34
\]
over the full $K$-coordinate hypercube, then, for a constant $C_\alpha>0$ depending only on the
fixed level $\alpha$,
\[
\sum_{c=1}^K e^{-C_\alpha\varepsilon^2 n_c}\le4\log\frac43.
\]
Hence
\[
\sum_c n_c=\Omega(K\varepsilon^{-2}\log K),
\]
at least $K/2$ regions have $n_c=\Omega(\varepsilon^{-2}\log K)$, and a uniform quota has
$n_c=\Omega(\varepsilon^{-2}\log K)$.
\end{lemma}

\subsection*{(c) Necessity: a perturbative two point lower bound}
\emph{Construction.} Let $X\sim\mathrm{Unif}[0,1]$ under every target law and take
$s(x,c)=x$. For $a\in(-1,1)$ define
\begin{align*}
P_a(Y=c\mid X=x)&=\frac12+a\left(\frac12-x\right),\\
P_a(Y=0\mid X=x)&=\frac12-a\left(\frac12-x\right).
\end{align*}
Both label probabilities lie strictly between zero and one. Also $P_a(Y=c)=1/2$, and the
class-$c$ conditional score CDF is
\begin{align}
F_a(t)
&=P_a(X\le t\mid Y=c)\notag\\
&=2\int_0^t\left\{\frac12+a\left(\frac12-x\right)\right\}\,dx\notag\\
&=t+a(t-t^2),\qquad 0\le t\le1.
\label{eq:two_point_cdf}
\end{align}
Its derivative is $1+a(1-2t)\ge1-|a|>0$. Thus its $(1-\alpha)$-quantile $q(a)$ is unique and solves
\[
q(a)+a\{q(a)-q(a)^2\}=1-\alpha.
\]
Implicit differentiation yields
\begin{equation}
q'(a)=-\frac{q(a)-q(a)^2}{1+a\{1-2q(a)\}}.
\label{eq:q_derivative}
\end{equation}
In particular $q'(0)=-\alpha(1-\alpha)$. By continuity, there are constants
$a_0,d_\alpha>0$ such that
\[
-q'(a)\ge d_\alpha
\quad\text{for every }|a|\le a_0.
\]

Choose a constant $c_1>1/d_\alpha$, set $\tau=c_1\varepsilon$, and restrict
$\varepsilon\le a_0/c_1$. Compare $P_+=P_{+\tau}$ and $P_-=P_{-\tau}$. They have the same
$P_T(X)$; take the source law to be the $a=0$ law under both hypotheses. The unbounded unlabeled
pool and the source therefore have identical distributions. The quantile separation satisfies
\begin{align}
\Delta
&=q(-\tau)-q(+\tau)\notag\\
&=\int_{-\tau}^{+\tau}\{-q'(a)\}\,da\notag\\
&\ge2d_\alpha\tau
>2\varepsilon.
\label{eq:two_point_separation}
\end{align}

\emph{Reduction in full.} Let a threshold procedure output $\hat q_c$. Under $P_a$, its class $c$
part of the common success event is
\[
A_a=
\left\{
F_a(\hat q_c)\ge1-\alpha,\ 
|\hat q_c-q(a)|\le\varepsilon
\right\}.
\]
Since $F_a$ is strictly increasing and $F_a(q(a))=1-\alpha$, validity gives
$\hat q_c\ge q(a)$. Hence
\begin{equation}
A_a\quad\Longrightarrow\quad
q(a)\le\hat q_c\le q(a)+\varepsilon.
\label{eq:two_point_interval}
\end{equation}
Define the test
\[
\widehat a=+\tau
\quad\Longleftrightarrow\quad
\hat q_c<\frac{q(+\tau)+q(-\tau)}2.
\]
Under $P_+$, equations \eqref{eq:two_point_separation} and \eqref{eq:two_point_interval} give
\[
\hat q_c\le q(+\tau)+\varepsilon
<q(+\tau)+\frac{\Delta}{2}
=\frac{q(+\tau)+q(-\tau)}2,
\]
so the test declares $+\tau$. Under $P_-$, validity gives
\[
\hat q_c\ge q(-\tau)
>\frac{q(+\tau)+q(-\tau)}2,
\]
so the test declares $-\tau$. The test can err under $P_a$ only on $A_a^c$. Since the theorem's
simultaneous event implies $A_a$, success probability at least $3/4$ under both hypotheses would
produce a test with each error probability at most $1/4$.

\emph{Information bound.} Write $v(x)=1/2-x$. Conditional on $X=x$, the two hypotheses are
Bernoulli with
\[
p_+(x)=\frac12+\tau v(x),
\qquad
p_-(x)=\frac12-\tau v(x).
\]
For $\tau\le1/2$, both probabilities lie in $[1/4,3/4]$. The elementary Bernoulli bound
$\mathrm{kl}(p,q)\le(p-q)^2/\{q(1-q)\}$ gives
\begin{align*}
\mathrm{KL}(P_+\|P_-)
&\le\frac{64}{3}\tau^2\int_0^1v(x)^2\,dx\\
&=\frac{16}{9}\tau^2.
\end{align*}
For $m$ i.i.d.\ labeled audit pairs, Pinsker's inequality and tensorization imply
\[
\mathrm{TV}(P_+^{\otimes m},P_-^{\otimes m})
\le\sqrt{\frac{m}{2}\mathrm{KL}(P_+\|P_-)}
\le\sqrt{\frac{8m\tau^2}{9}}.
\]
If
\[
m\le\frac{9}{128c_1^2}\varepsilon^{-2},
\]
then this total variation distance is at most $1/4$. The source and unlabeled observations are
identical under the hypotheses, so they add zero total variation. Every test must consequently
have combined error at least
\[
1-\mathrm{TV}(P_+^{\otimes m},P_-^{\otimes m})\ge\frac34.
\]
This contradicts combined error at most $1/2$. In fact one law has failure probability at least
$3/8$, which proves the stated $1/4$ lower bound with
$c_0=9/(128c_1^2)$. \hfill$\square$

\subsection*{(d) Simultaneous necessity: the $\log K$ lower bound}
\emph{Construction.} Let
\[
X=(Z,U),\qquad
Z\sim\mathrm{Unif}\{1,\ldots,K\},\qquad
U\sim\mathrm{Unif}[0,1],
\]
with $Z$ observed and $Z\perp U$. The label set is $\{0,1,\ldots,K\}$, with $0$ a background
class. For a vector $a=(a_1,\ldots,a_K)\in\{-\tau,+\tau\}^K$, set, in region $Z=c$,
\begin{align*}
P_a(Y=c\mid Z=c,U=u)&=\frac12+a_c\left(\frac12-u\right),\\
P_a(Y=0\mid Z=c,U=u)&=\frac12-a_c\left(\frac12-u\right).
\end{align*}
The foreground scores are
\[
s((z,u),c)=
\begin{cases}
u,&z=c,\\
M,&z\ne c,
\end{cases}
\qquad M>1,
\]
and $s(\cdot,0)=M$. Take the source law to be the $a=0$ law. Every hypothesis has the same target
covariate marginal and the same source law. Moreover,
\[
P_a(Y=c)=\frac1K\int_0^1
\left\{\frac12+a_c\left(\frac12-u\right)\right\}\,du
=\frac1{2K}.
\]
Conditional on $Y=c$, necessarily $Z=c$, and direct integration gives
\begin{align}
F_{a_c}(t)
&=P_a\{s(X,c)\le t\mid Y=c\}\notag\\
&=t+a_c(t-t^2),\qquad 0\le t\le1.
\label{eq:hypercube_conditional_cdf}
\end{align}
Thus the oracle threshold is the same function $q(a_c)$ used in part (c).
For $a\ne0$ it is explicitly
\[
q(a)=
\frac{1+a-\sqrt{(1+a)^2-4a(1-\alpha)}}{2a},
\qquad
q(0)=1-\alpha.
\]

The marginal score CDF, which governs the contribution of class $c$ to total expected set size, is
\begin{equation}
G_c(t)=P_T\{s(X,c)\le t\}
=
\begin{cases}
0,&t<0,\\
t/K,&0\le t\le1,\\
1/K,&1<t<M,\\
1,&t\ge M.
\end{cases}
\label{eq:hypercube_marginal_cdf}
\end{equation}
Consequently, if
\[
\Delta=q(-\tau)-q(+\tau)>0,
\]
then changing the foreground threshold from $q(+\tau)$ to $q(-\tau)$ changes expected set size by
\begin{equation}
G_c(q(-\tau))-G_c(q(+\tau))=\frac{\Delta}{K}.
\label{eq:hypercube_size_gap}
\end{equation}
This is the factor that prevents an unnormalized set-size criterion from identifying a coordinate.

\emph{Reduction in full.} Choose $\tau=c_1\varepsilon$ with $c_1$ fixed so that, for all
sufficiently small $\varepsilon$,
\[
\Delta=q(-\tau)-q(+\tau)>2\varepsilon.
\]
Such a choice exists because
$\Delta=2\alpha(1-\alpha)\tau+O(\tau^3)$. The common efficiency criterion is
\[
\max_{1\le c\le K}|\hat q_c-q(a_c)|\le\varepsilon.
\]
On the event $\mathcal V(P_a)\cap\mathcal E_\varepsilon(P_a)$, strict monotonicity of
$F_{a_c}$ turns the criterion and validity into the explicit coordinatewise interval
\begin{equation}
q(a_c)\le\hat q_c\le q(a_c)+\varepsilon,
\qquad c=1,\ldots,K.
\label{eq:hypercube_efficiency_interval}
\end{equation}
Define
\[
\widehat a_c=+\tau
\quad\Longleftrightarrow\quad
\hat q_c<\frac{q(+\tau)+q(-\tau)}2.
\]
If $a_c=+\tau$, then \eqref{eq:hypercube_efficiency_interval} and $\varepsilon<\Delta/2$ give
\[
\hat q_c\le q(+\tau)+\varepsilon
<\frac{q(+\tau)+q(-\tau)}2,
\]
so $\widehat a_c=+\tau$. If $a_c=-\tau$, validity in
\eqref{eq:hypercube_efficiency_interval} gives
\[
\hat q_c\ge q(-\tau)
>\frac{q(+\tau)+q(-\tau)}2,
\]
so $\widehat a_c=-\tau$. Therefore
\[
\mathcal V(P_a)\cap\mathcal E_\varepsilon(P_a)
\subseteq
\{\widehat a_c=a_c\text{ for every }c\}.
\]
The sign vector is forced by the repaired criterion.

\emph{Product testing experiment.} Give the procedure $n_c$ labeled observations from region
$Z=c$, with quotas fixed before seeing their labels. The region data are independent across $c$.
Within region $c$, one observation has law $Q_{a_c}$ for $(U,Y)$. The Hellinger affinity of
$Q_{+\tau}$ and $Q_{-\tau}$ is
\begin{align*}
\rho_1
&=\int_0^1\left[
\sqrt{\left(\frac12+\tau v\right)\left(\frac12-\tau v\right)}
+\sqrt{\left(\frac12-\tau v\right)\left(\frac12+\tau v\right)}
\right]du\\
&=\int_0^1\sqrt{1-4\tau^2(1/2-u)^2}\,du\\
&=1-\eta.
\end{align*}
For $\tau\le1$, the inequalities
$x/2\le1-\sqrt{1-x}\le x$ for $0\le x\le1$ yield
\[
\frac{\tau^2}{6}\le\eta\le\frac{\tau^2}{3}.
\]
With $n_c$ independent region observations, the affinity is
$\rho_{n_c}=(1-\eta)^{n_c}$.

Place the uniform product prior on $a\in\{-\tau,+\tau\}^K$. The likelihood and prior both factor
over coordinates, so the posterior factorizes. The Bayes-optimal estimator for exact vector
recovery is coordinatewise MAP, and its all-correct probability is
\[
\prod_{c=1}^K(1-p_c^\star),
\]
where $p_c^\star$ is the equal-prior Bayes error for testing the two region-$c$ laws. No vector
estimator has larger prior-average exact-recovery probability. A worst-case success probability of
$3/4$ for quantile recovery therefore implies
\begin{equation}
\prod_{c=1}^K(1-p_c^\star)\ge\frac34.
\label{eq:product_success}
\end{equation}

The affinity and total variation inequality give
\begin{align*}
p_c^\star
&=\frac{1-\mathrm{TV}(Q_{+\tau}^{\otimes n_c},
Q_{-\tau}^{\otimes n_c})}{2}\\
&\ge\frac{1-\sqrt{1-\rho_{n_c}^2}}2\\
&\ge\frac{\rho_{n_c}^2}{4}\\
&=\frac14(1-\eta)^{2n_c}.
\end{align*}
Since $\eta\le\tau^2/3\le1/2$ and $\log(1-\eta)\ge-2\eta$,
\[
p_c^\star
\ge\frac14e^{-4\eta n_c}
\ge\frac14e^{-C_\alpha\varepsilon^2 n_c},
\qquad
C_\alpha=\frac{4c_1^2}{3}.
\]
Taking logarithms in \eqref{eq:product_success} and using
$\log(1-x)\le-x$ gives
\[
\sum_{c=1}^Kp_c^\star\le\log\frac43.
\]
It follows that
\begin{equation}
\sum_{c=1}^K e^{-C_\alpha\varepsilon^2n_c}
\le4\log\frac43=:A.
\label{eq:exponential_budget_constraint}
\end{equation}

\emph{Extracting the $\log K$ rate.} Put
$y_c=e^{-C_\alpha\varepsilon^2n_c}$. Jensen's inequality for the convex function
$-\log y$ and \eqref{eq:exponential_budget_constraint} give
\begin{align*}
\sum_{c=1}^K n_c
&=\frac1{C_\alpha\varepsilon^2}\sum_{c=1}^K\log\frac1{y_c}\\
&\ge\frac{K}{C_\alpha\varepsilon^2}
\log\frac{K}{\sum_cy_c}\\
&\ge\frac{K}{C_\alpha\varepsilon^2}\log\frac KA
=\Omega(K\varepsilon^{-2}\log K).
\end{align*}
If at least $K/2$ coordinates had
\[
n_c<\frac1{C_\alpha\varepsilon^2}\log\frac{K}{2A},
\]
their $y_c$ values would sum to more than $A$, contradicting
\eqref{eq:exponential_budget_constraint}. Hence at least $K/2$ regions have
$n_c=\Omega(\varepsilon^{-2}\log K)$.

Finally, the number $M_c$ of foreground labels $Y=c$ among the $n_c$ region observations is
$\mathrm{Binomial}(n_c,1/2)$, and its distribution does not depend on $a_c$. Standard Chernoff
bounds give
\[
P\left\{\frac{n_c}{3}\le M_c\le\frac{2n_c}{3}\right\}
\ge1-2e^{-n_c/54}.
\]
Thus the regional paid-label budget and the number of usable class-$c$ audit scores differ only by
constant factors with high probability in the lower-bound regime. PAC Audit Mondrian applied to
those foreground scores attains the upper rate from part (b), which establishes matching rates for
simultaneous quantile recovery under this balanced construction. \hfill$\square$

\begin{remark}[Scope of the repaired theorem]
Validity is the single PAC event $\mathcal V(P)$ in all four parts. Part (b) uses a local density
lower bound to convert CDF error into threshold error. Parts (c) and (d) apply to all classwise
threshold procedures. The matching statement concerns class conditional quantile recovery. The
expected-size result is the one-sided corollary above, with each marginal sensitivity $L_c$
visible.
\end{remark}

\section{Joint accept and err risk control (negative control support)}
\label{supp:crc}

The CRC guarantee applies to the margin abstention negative control (main paper, method section).
It controls a \emph{marginal joint} risk, which is weaker than per class conditional coverage, and
this is precisely why margin abstention leaves per class undercoverage unresolved. The CRC
threshold requires a \textbf{labeled target pool}, so this result does not contribute a deployable
method.

\begin{proposition}[CRC joint risk control]
\label{prop:crc}
Let $\{(x_i,y_i)\}_{i=1}^n$ be a labeled target calibration sample exchangeable with a test
point $(x^\star,y^\star)$. Define the threshold indexed per point loss
\[
L_i(t)=\mathbf{1}\{\sig_{\mathrm{mar}}(x_i)<t\}\cdot\mathbf{1}\{y_i\notin\hat{C}(x_i)\}
\]
(accept and err: monotone non decreasing in $t$). Let $\hat{t}$ be the largest threshold satisfying
\begin{equation}
\label{eq:crc}
\frac{n\,\widehat{R}_n(\hat{t})+B}{n+1}\ \le\ \delta,
\qquad \widehat{R}_n(t)=\tfrac1n\sum_{i=1}^{n}L_i(t),
\end{equation}
with $B{=}1$ and $\delta{=}\alpha$. Then $E[L(\hat{t})]\le\alpha$ on a fresh exchangeable test
point.
\end{proposition}

\noindent This is the Conformal Risk Control guarantee of \citet{angelopoulos2023crc}. The
guarantee is on a \emph{joint marginal} risk and does not provide per class conditional coverage.
It also requires target labels for threshold selection.
Margin abstention therefore serves as a diagnostic negative control and is not a deployable method.

\section{The LE chart is isometric}
\label{supp:isometry}

\begin{lemma}[Isometric vectorization]
\label{lem:isometry}
The map
\[
\Phi(X)=\vech_{\!\sqrt2}(\Log X)
\]
from $(\SPD(d),\dLE)$ to $(\R^{d(d+1)/2},\|\cdot\|_2)$ is an isometry:
\[
\|\Phi(X)-\Phi(Y)\|_2=\|\Log X-\Log Y\|_F=\dLE(X,Y).
\]
Consequently: (i) the
min distance signal $\sig_{\mathrm{ood}}$ and geodesic margin $\sig_{\mathrm{mar}}$ computed
from $\Phi$ equal their log Euclidean manifold counterparts exactly; (ii) all backbone computations
(nearest mean softmax, tangent logistic, density ratio discriminator) operate in the isometric LE
chart without additional geometric approximation.
\end{lemma}

\noindent The $\sqrt2$ weighting on off diagonal entries makes the half vectorization norm preserving
on symmetric matrices; the result follows from $\dLE(X,Y)=\|\Log X-\Log Y\|_F$.

\begin{corollary}[Inherited invariances, and their limits]
\label{cor:inv}
Because $\dLE$ is invariant under congruence by an orthogonal matrix ($X\mapsto OXO^\top$,
$O\in O(d)$) and under inversion ($X\mapsto X^{-1}$), all abstention signals inherit these
invariances. They are not invariant under the full $\GL(d)$ congruence action; that property belongs
to the affine invariant metric (AIRM). A fully affine invariant variant is future work.
\end{corollary}

\begin{remark}[Honest theoretical status]
\label{rem:honestscope}
Weighted CP inherits the guarantees of \citet{tibshirani2019,barber2023} only to the extent the
covariate shift assumption holds, which is approximate here since the shift acts on $p(y\mid x)$,
and this is why it recovers only by over covering. Source Mondrian's guarantee is the main paper's
Proposition~1, approximate under shift (the main paper's Remark~1); margin abstention's is the
marginal joint risk CRC control of Proposition~\ref{prop:crc} above. We make no claim of conditional
coverage for any method, no $\GL(d)$ invariance, and no asymptotic optimality of any signal; by the
main paper's Proposition~2, the efficiency limit under joint shift is a boundary inherent to the
problem, and every method faces it.
\end{remark}

\section{Method and calibration details}

\paragraph{Computing infrastructure.}
Backbone training runs on a single NVIDIA A5000 on an internal cluster. Conformal
calibration and every evaluation reported in this paper are post hoc and run on CPU: they
consume cached descriptors or logits and require one sort per class, so the full six method
comparison over ten seeds completes in minutes without a GPU.

\label{supp:method}

This section collects the formal definitions, constants, and formulas underlying the four
calibration methods of the main paper's method section.

\paragraph{SPD descriptors and backbone configurations.}
Each input sequence is summarized by an SPD descriptor $\varphi(x)\in\SPD(d)$, the temporal
covariance of joint coordinates and velocities. The three backbone configurations are:
(i)~\textbf{nearest mean}, raw skeleton SPD descriptors ($d{=}150$) classified by a log Euclidean
nearest class mean rule (softmax over negative geodesic distances to class Karcher means; formula
below); (ii)~\textbf{tangent logistic}, raw skeleton SPD ($d{=}150$) classified by a tangent space
logistic classifier; (iii)~\textbf{ST-GCN features}, per frame ST-GCN features
\citep{yan2018stgcn} summarized into a temporal covariance SPD descriptor ($d{=}64$) classified by
the same tangent space logistic classifier. The ST-GCN-feature configuration is run in two
training regimes, a $40$-epoch and an $80$-epoch regime; the
resulting worst class coverage across all four backbone rows appears in
Table~\ref{tab:backbone_sweep} (Section~\ref{supp:backbone_sweep}).

Source data is partitioned into disjoint scorer training and calibration subsets: the backbone
classifier (class means or logistic weights) is fit on the former, and conformal quantiles are
estimated on the latter, at a per class calibration count of approximately $334$ on NTU-60
cross subject. All four calibration methods share this backbone and calibration pool.

\paragraph{Karcher means and the isometric vectorization.}
For each class $c$, the log Euclidean Karcher mean is
\[
\Mc = \Exp\!\Big(\tfrac{1}{|S_c|}\sum_{i\in S_c}\Log\varphi(x_i)\Big),
\]
computed on the scorer training subset. The LE vectorization $\Phi(X)=\vech_{\!\sqrt2}(\Log X)$,
a half vectorization that scales off diagonal entries by $\sqrt2$, is an isometry: its Euclidean
norm equals the Frobenius norm of $\Log X$ (Lemma~\ref{lem:isometry}, Section~\ref{supp:isometry}), so
all backbone computations live in an isometric copy of the LE manifold.

\paragraph{The LAC nonconformity score.}
All four calibration methods use the LAC nonconformity score \citep{sadinle2019lac}:
$s(x,c)=1-\hat{p}(c\mid x)$, where $\hat{p}(\cdot\mid x)$ is the backbone's class probability
output. For the nearest mean configuration,
\[
\hat{p}(c\mid x)=\frac{\exp(-\dLE(\varphi(x),\Mc)/\tau)}{\sum_{c'}\exp(-\dLE(\varphi(x),M_{c'})/\tau)},
\qquad \tau{=}0.5,
\]
so geodesic distance enters indirectly through the softmax; for the tangent logistic
configuration, $\hat{p}$ is the logistic classifier output on $\Phi(\varphi(x))$.

\paragraph{Source Mondrian per class quantile.}
For each class $c$,
\begin{equation}
\label{eq:mondrian_q}
\hat{q}_c = \text{the } \lceil(n_c+1)(1-\alpha)\rceil\text{-th smallest element of }
  \{s(x_i,c) : y_i = c,\ i=1,\ldots,n\},
\end{equation}
where $n_c=|\{i:y_i=c\}|$ is the per class calibration count (approximately $334$ per class on
NTU-60 cross subject), $\hat q_c=+\infty$ whenever the index $\lceil(n_c+1)(1-\alpha)\rceil$
exceeds $n_c$, and the prediction set is $\hat{C}(x)=\{c:s(x,c)\le\hat{q}_c\}$. At this
$n_c$, the finite sample correction $1/(n_c+1)\approx0.003$ is negligible.

\paragraph{Weighted conformal quantile.}
The marginal weighted quantile, using a $+1$ notional test atom, is
\begin{equation}
\label{eq:wq}
Q_{1-\alpha}\big(\{s_i\},\{w_i\}\big)
=\inf\Big\{q:\ \tfrac{\sum_{i:\,s_i\le q} w_i}{\sum_j w_j + 1}\ \ge\ 1-\alpha\Big\}.
\end{equation}
The exact per test point variant \citep{tibshirani2019} normalizes the calibration weights in
Equation~\eqref{eq:wq} by $w(x^\star)$ for each test point $x^\star$; the test point itself
contributes the notional unit atom, placed at $+\infty$, so it enters the denominator of
Equation~\eqref{eq:wq} but never the numerator at a finite threshold. We report this exact variant throughout; the marginal
single threshold variant fails to recover coverage on our controlled synthetic study
($0.704/0.729$; Table~\ref{tab:coverage}, Section~\ref{app:h3}).

A weighted class conditional variant combines density ratio weights and per class quantiles: for
each class $c$ it computes the marginal weighted quantile of Equation~\eqref{eq:wq} over the class
$c$ calibration scores $\{s(x_i,c):y_i=c\}$ with weights $w(x_i)$ (one threshold per class, without
the per test point normalization), in place of the unweighted order statistic of
Equation~\eqref{eq:mondrian_q}.

\paragraph{The density ratio discriminator.}
Importance weights $w(x)\approx p_{\mathrm{target}}(x)/p_{\mathrm{source}}(x)$ are SPD-derived. We
fit an $\ell_2$-regularized logistic discriminator ($C{=}1$, balanced classes) on
$\Phi$-vectorized features to separate source from target; the resulting ratio
$w(x)=p(\text{target}\mid x)/p(\text{source}\mid x)$ is clipped to $[0,20]$, fit on a disjoint
pool, and applied out of sample.

\paragraph{Margin-abstention signals.}
We study two geometric per sample abstention signals: the min distance OOD signal
$\sig_{\text{ood}}(x)=\min_c \dg(\varphi(x),\Mc)$ and the geodesic margin
$\sig_{\text{mar}}(x)=\dg(\varphi(x),M_{(1)})-\dg(\varphi(x),M_{(2)})\le 0$, where
$M_{(1)},M_{(2)}$ are the two nearest class manifolds and geodesic distances are computed via
$\Phi$ (Lemma~\ref{lem:isometry}, Section~\ref{supp:isometry}). The signed margin is nonpositive:
strongly negative values mean a confidently nearest class, values near zero mean ambiguity, and
prose statements such as ``large margin'' refer to its magnitude
$|\sig_{\text{mar}}(x)|$. The margin signal is thresholded by
Conformal Risk Control (Proposition~\ref{prop:crc}, Section~\ref{supp:crc}), which requires a labeled
target calibration pool.

\section{Headline per class collapse, recovery frontier, and severity spectrum (full figures)}
\label{supp:headline_figures}

The main paper's teaser figure (Figure~1) summarizes the per class collapse and the recovery
frontier on the headline NTU-60 cross subject result. The three figures below give the full,
single panel versions, including the severity spectrum across all three real shifts.

\begin{figure}[t]
\centering
\includegraphics[width=0.65\linewidth]{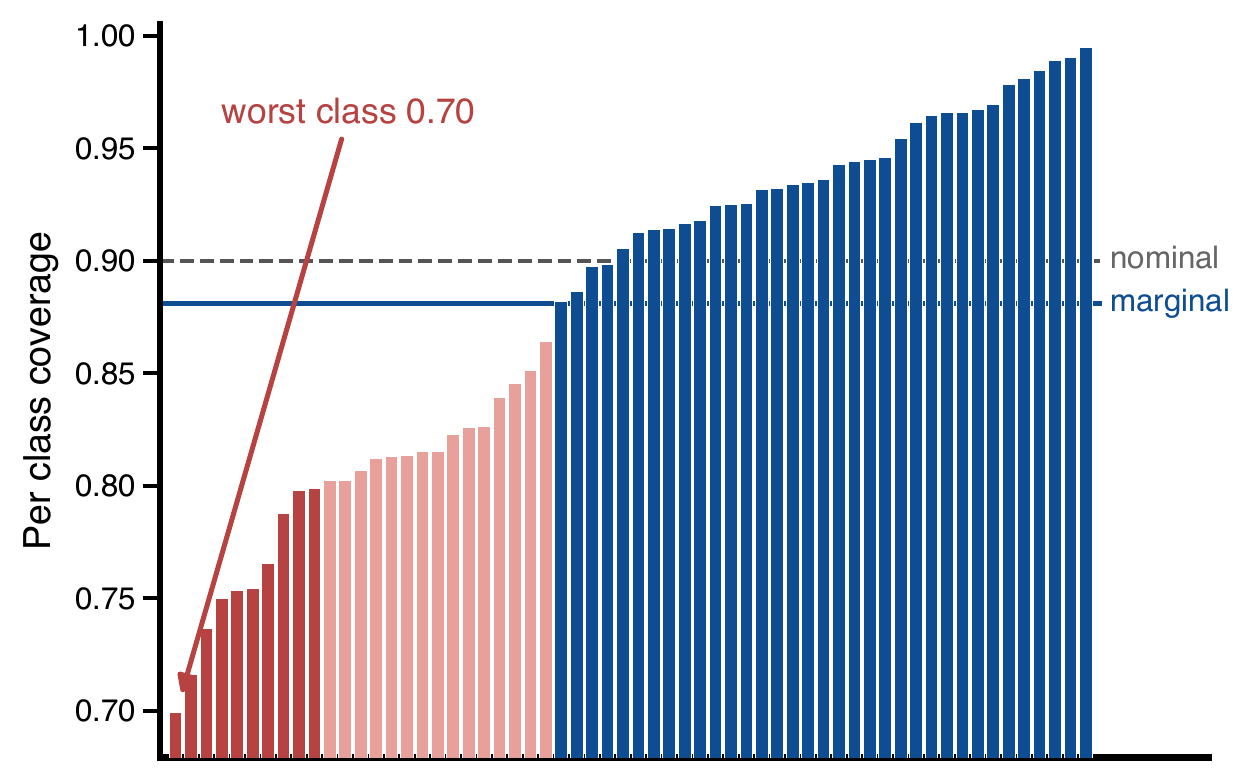}
\caption{Per class coverage on the real NTU-60 cross subject skeleton benchmark under split
conformal prediction. Classes are sorted by coverage. The marginal number sits near the nominal level while
a large group of classes falls into the unsafe band, the worst near seventy percent.}
\label{fig:conditional_collapse}
\end{figure}

\begin{figure}[t]
\centering
\includegraphics[width=0.6\linewidth]{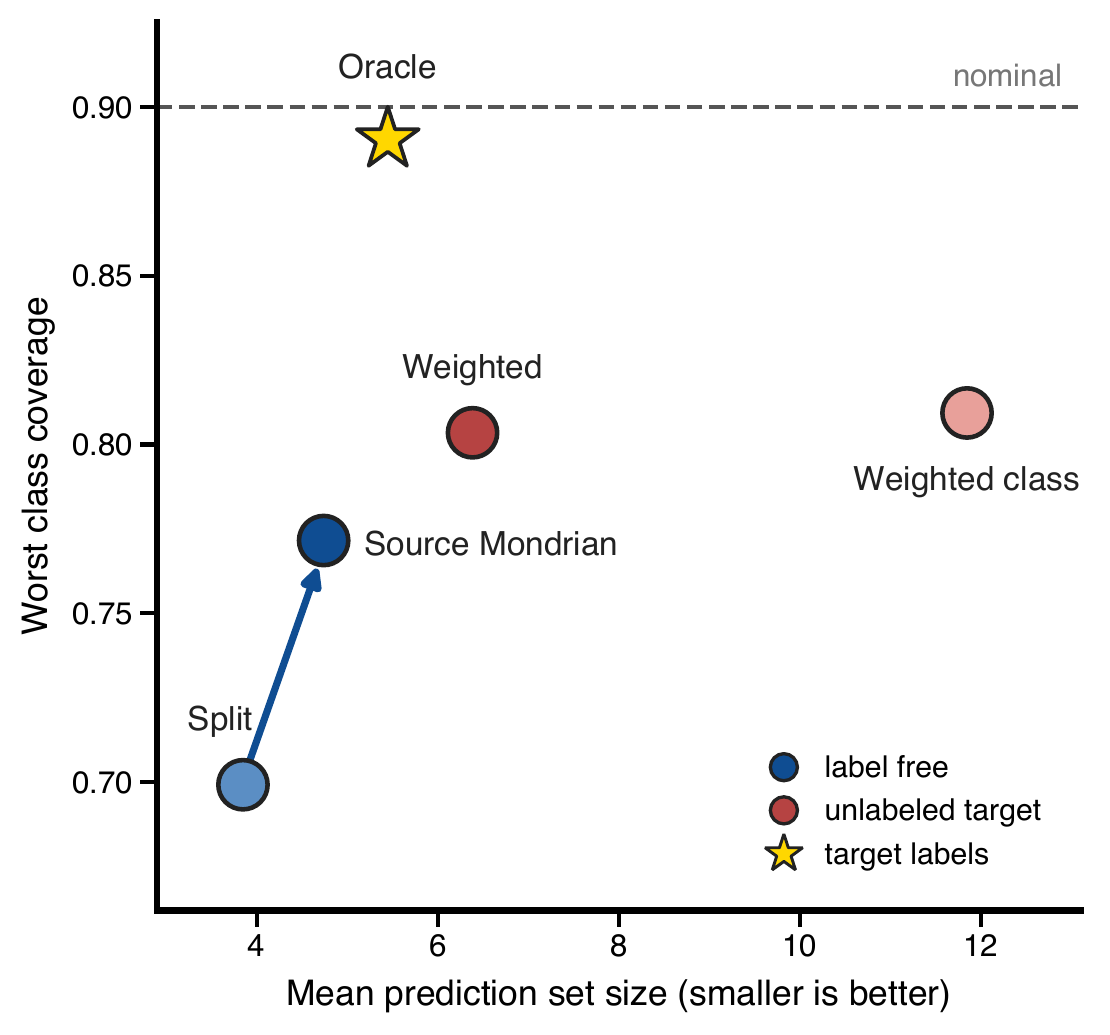}
\caption{The recovery frontier on the real NTU-60 cross subject skeleton benchmark. Each method is
placed by its worst class coverage and its mean prediction set size. Source Mondrian lifts the worst class
using source labels alone, at a small set size cost, and it holds marginal coverage on target. The
weighted methods reach a higher worst class only by inflating sets and overcovering the marginal;
Weighted class denotes the weighted class conditional combination.
The target label oracle marks the ceiling near the nominal line.}
\label{fig:frontier}
\end{figure}

\begin{figure}[t]
\centering
\includegraphics[width=0.65\linewidth]{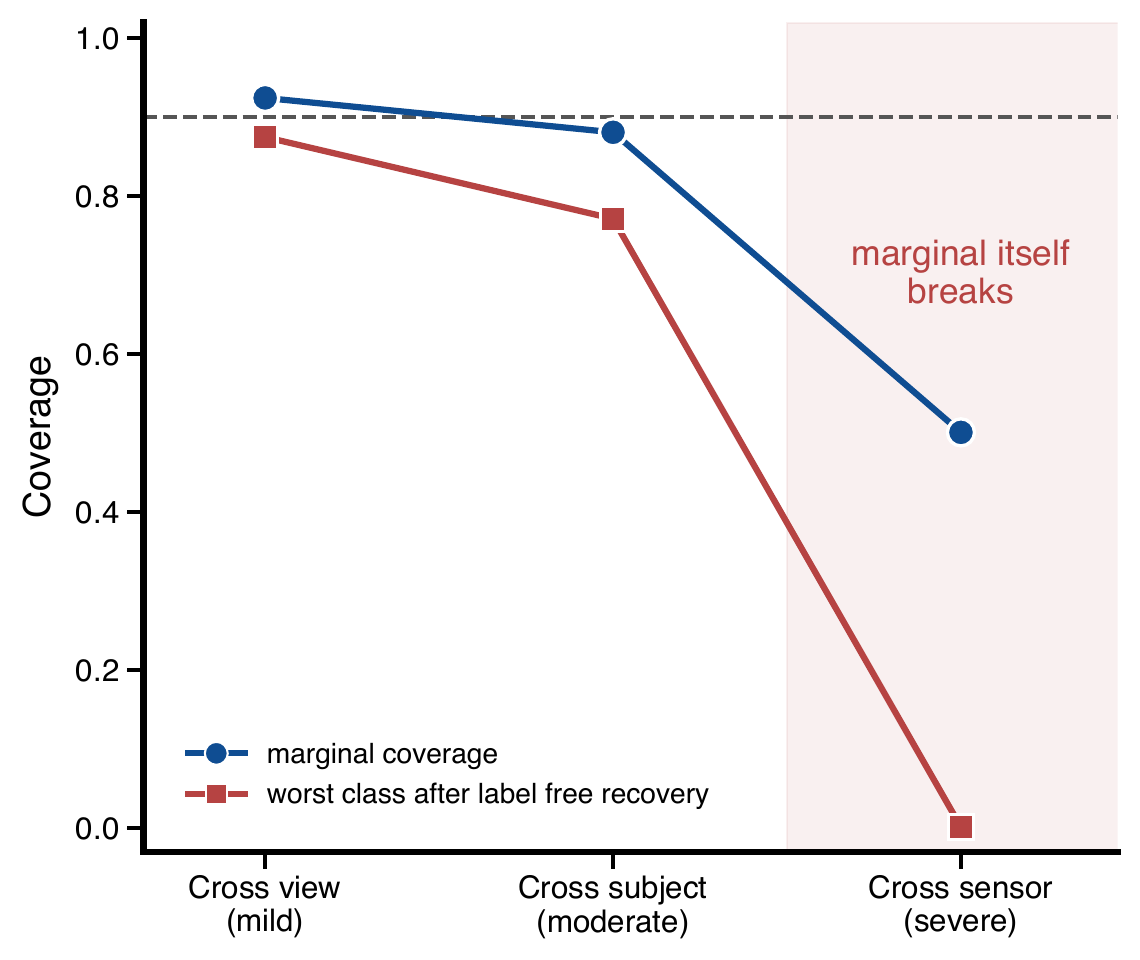}
\caption{The severity spectrum across three real NTU based shifts. Marginal coverage holds under
the mild and moderate shifts and then drops sharply under the severe one. The worst class
after label free recovery degrades in step and finally collapses. The shaded region marks where marginal
coverage itself breaks and the evaluated label free methods no longer recover per class coverage.}
\label{fig:spectrum}
\end{figure}

\section{Backbone-strength sweep}
\label{supp:backbone_sweep}

\paragraph{Important caveat.}
The sweep varies \emph{both} SPD representation \emph{and} classifier together; it is not a
controlled single variable ablation. The three backbone configurations are: nearest class mean on
raw skeleton SPD; tangent logistic on raw skeleton SPD; and tangent logistic on ST-GCN-feature SPD.
The ST-GCN-feature configuration is run in two training regimes ($40$-epoch and $80$-epoch),
giving four rows in Table~\ref{tab:backbone_sweep}.

\paragraph{Finding.}
As the combined representation+classifier becomes more discriminative (target accuracy from
${\sim}$chance to $0.73$ on the GCN head), prediction sets tighten (${\approx}27 \to 3.85$ of
$60$ classes; Figure~\ref{fig:backbone_sweep}). Source Mondrian reduces per class undercoverage at all tested levels and is the
only near nominal marginal, label free recoverer throughout. A retained result file backs the
conformal metrics of the strongest row only. The head accuracies, including the $0.73$ endpoint,
and every value in the three weaker rows come from runs whose outputs were not retained, so this
trend is descriptive and cannot be reproduced from the released artifacts.

\begin{table}[t]
\centering
\small
\caption{\textbf{[Real data, NTU-60 cross subject] Backbone sweep: worst class per class coverage.}
Representation and classifier vary jointly (not a single variable ablation). Bold: highest
non oracle worst class coverage per backbone row. $^\dagger$GCN head accuracy; conformal backbone
uses tangent logistic on SPD. $^\ddagger$Tangent-logistic on raw SPD. $^\circ$Threshold requires
labeled target pool. Set sizes approximate for nearest mean and tangent rows (split CP only
measured). $\alpha{=}0.10$. Provenance: the released main recovery result file backs the conformal
metrics and set sizes of the ST-GCN 80-epoch row. The ST-GCN head accuracies come from project notes
and appear in no result file, and no retained artifact backs the three weaker rows, so the cross
configuration pattern is descriptive and cannot be reproduced from the released artifacts.}
\label{tab:backbone_sweep}
\begin{tabular}{lcccccc}
\toprule
Backbone & split & source-CC & weighted & wCC & abstention$^\circ$ & oracle\\
\midrule
Nearest-mean (raw SPD) & 0.682 & 0.690 & \textbf{0.711} & 0.698 & 0.687$^{@92\%}$ & 0.888\\
\quad sets (split / source-CC) & \multicolumn{6}{l}{${\approx}27$ / n/a}\\[2pt]
Tangent-logistic (raw SPD$^\ddagger$, top-1$\approx$0.36) & 0.720 & \textbf{0.824} & 0.723 & 0.814 & 0.722 & 0.876\\
\quad sets (split / source-CC) & \multicolumn{6}{l}{${\approx}18$ / n/a}\\[2pt]
ST-GCN 40-epoch (GCN$^\dagger$ 0.635) & 0.693 & \textbf{0.798} & 0.717 & 0.605 & 0.681$^{@90\%}$ & 0.885\\
\quad sets (split / source-CC) & \multicolumn{6}{l}{$5.11$ / $7.87$}\\[2pt]
ST-GCN 80-epoch (GCN$^\dagger$ 0.727) & 0.699 & 0.772 & 0.803 & \textbf{0.809} & 0.700$^{@91\%}$ & 0.890\\
\quad sets (split / source-CC) & \multicolumn{6}{l}{$3.85$ / $4.74$}\\
\bottomrule
\end{tabular}
\end{table}

\begin{figure}[t]
\centering
\includegraphics[width=\linewidth]{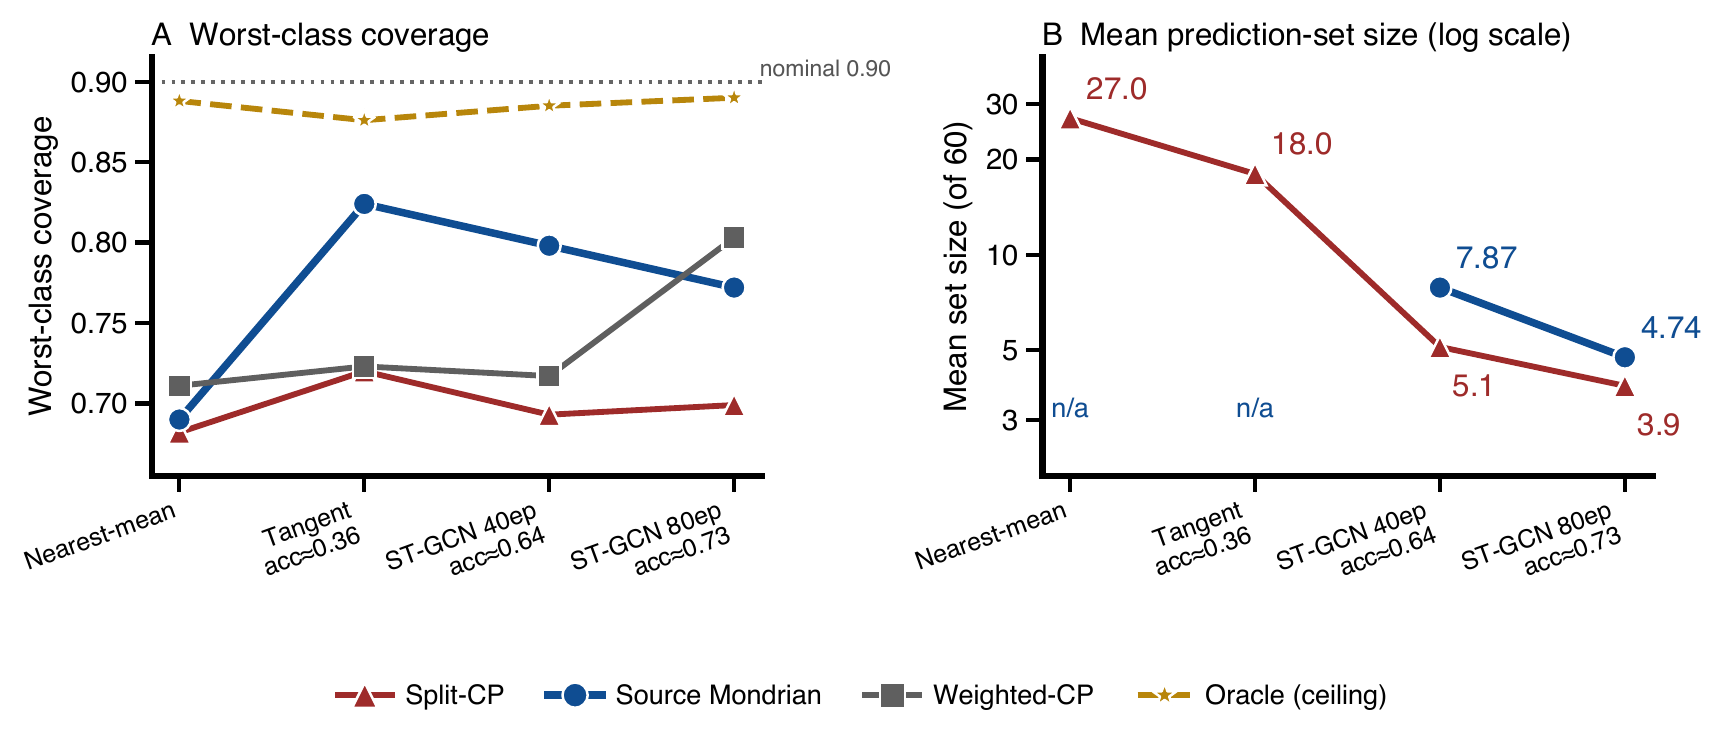}
\caption{\textbf{[Real data, NTU-60 cross subject] Backbone sweep.} Worst-class per class coverage
by method (Table~\ref{tab:backbone_sweep}). Representation and classifier vary jointly.}
\label{fig:backbone_sweep}
\end{figure}

Table~\ref{tab:recovery} gives the full six method breakdown for the main recovery experiment on
the strongest (ST-GCN 80-epoch) backbone, and Figure~\ref{fig:recovery} shows worst class coverage
and the share of severely undercovered classes per method.

\begin{table}[t]
\centering
\small
\caption{\textbf{[Real data, NTU-60 cross subject, ST-GCN] Six method recovery, main experiment.}
Tangent-space SPD conformal on ST-GCN 80-epoch features (conformal top-1 $0.627$). $\alpha{=}0.10$,
$10$ seeds, $60$ classes, nominal $0.90$. Split CP holds marginal coverage yet $10$ of $60$ classes
fall below $0.80$ per class; source Mondrian recovers label free at a small set size cost; the
weighted methods raise the worst class only by marginal over coverage and larger sets; margin
abstention does not materially improve the worst class. $^\circ$Margin abstention's CRC threshold
needs a labeled target pool. $^\ast$Oracle needs target labels (ceiling).}
\label{tab:recovery}
\begin{tabular}{lcccc}
\toprule
Method & Marginal cov. & Worst-class cov. & Mean set size & Classes ${<}0.80$ (of 60)\\
\midrule
Split CP (baseline)                       & 0.881 & 0.699 & 3.85  & 10\\
Source Mondrian (ours, label free)        & 0.881 & 0.772 & 4.74  & 1\\
Weighted CP                               & 0.928 & 0.803 & 6.38  & 0\\
Weighted class conditional                & 0.909 & 0.809 & 11.85 & 0\\
Margin abstention$^\circ$ ($91\%$ acc.)   & 0.889 & 0.700 & 3.69  & 8\\
\textbf{Target-oracle class cond.}$^\ast$ & \textbf{0.906} & \textbf{0.890} & \textbf{5.45} & \textbf{0}\\
\bottomrule
\end{tabular}
\end{table}

\begin{figure}[t]
\centering
\includegraphics[width=\linewidth]{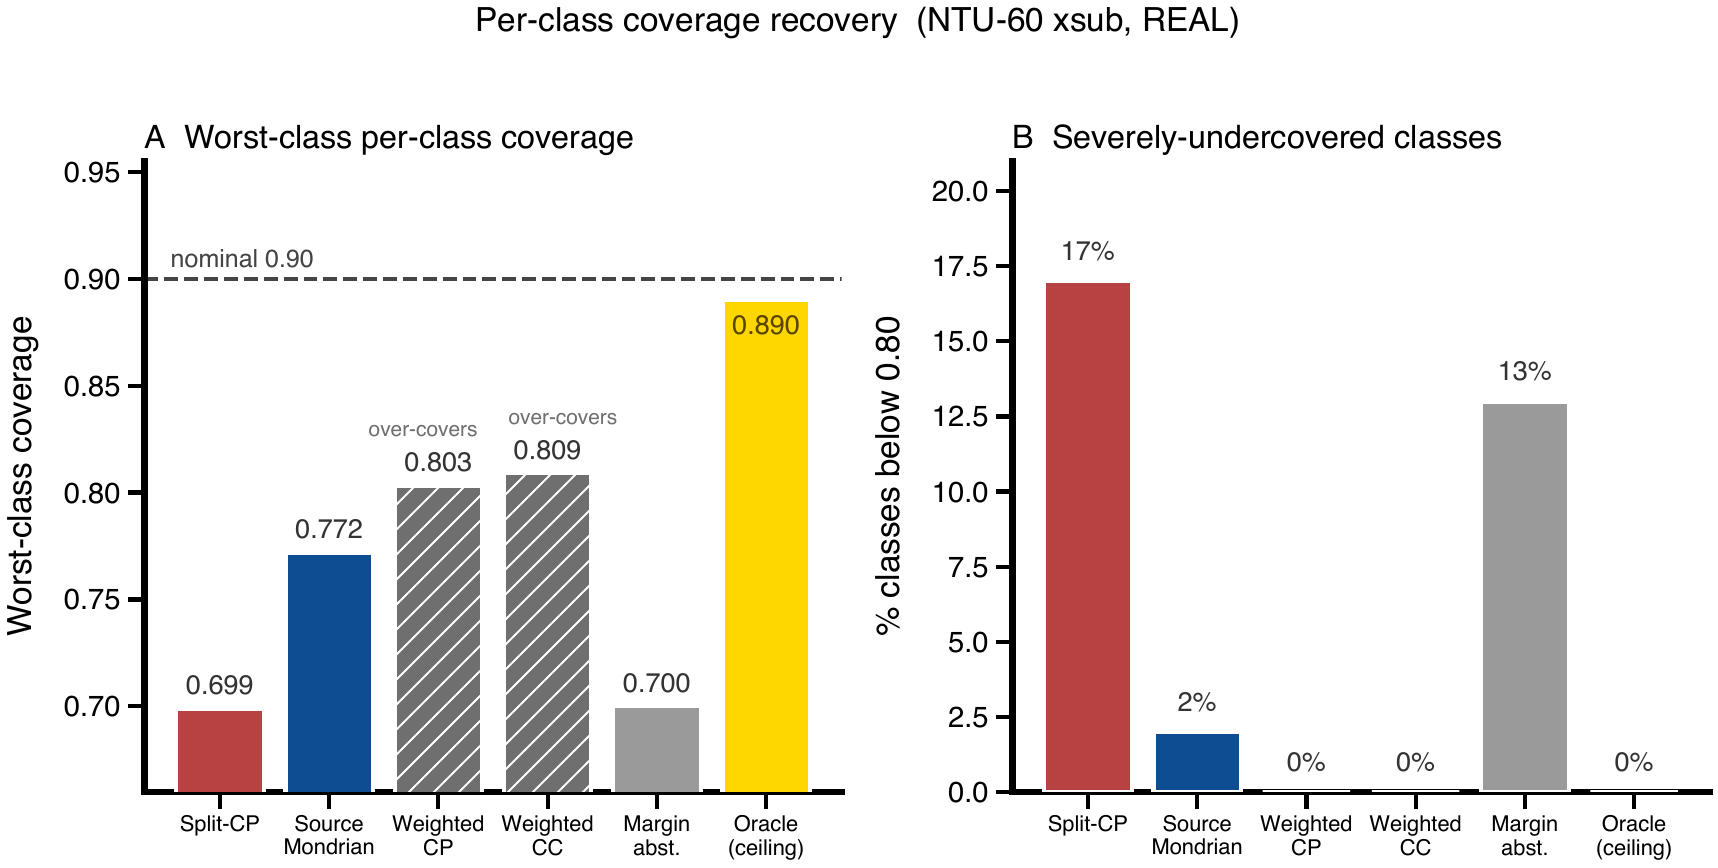}
\caption{\textbf{[Real data, NTU-60 cross subject] Worst-class coverage (left) and the percentage
of classes below $0.80$ coverage (right), by method (Table~\ref{tab:recovery}).} Source Mondrian
is the efficient, near nominal marginal recoverer.}
\label{fig:recovery}
\end{figure}

\subsection{Two estimands of worst-class coverage}
\label{supp:seed_dispersion}

Every worst-class coverage number in this paper is a minimum over per-class coverages estimated
across $10$ calibration seeds, and the minimum can be taken in two different orders. Estimand
(i) averages each class's coverage over seeds and then takes the minimum over classes; every
table above reports this estimand. Estimand (ii) takes the minimum over classes within each
seed and then averages that per-seed minimum over the $10$ seeds, with its standard deviation
and per-seed range. A class that underperforms on one seed and recovers on the rest can still
clear estimand (i) while it drags down the per-seed minimum feeding estimand (ii).

On the main NTU-60 cross-subject experiment (Table~\ref{tab:recovery}), split CP reads $0.699$
under estimand (i) and $0.677\pm0.029$ under estimand (ii), per-seed range $[0.635,0.717]$;
source Mondrian reads $0.772$ under estimand (i) and $0.739\pm0.024$ under estimand (ii), range
$[0.679,0.771]$ (Table~\ref{tab:seed_dispersion}). Across all $15$ artifacts in this paper that
store per-seed per-class coverage ($57$ method rows in total), estimand (i) meets or exceeds
estimand (ii) in every row and is strictly larger in $47$ of them. Estimand (i) is therefore the
larger of the two numbers everywhere it can be measured, and it is the one this paper reports
throughout. Estimand (ii) is the more pessimistic of the two, so the worst-class numbers this
paper reports understate the collapse slightly. The reported dispersion (mean $\pm$ sd in
Table~\ref{tab:seed_dispersion}) is the population standard deviation across the ten seeds.

\begin{table}[t]
\centering
\small
\caption{\textbf{[Real data, NTU-60 cross subject, ST-GCN] Worst-class coverage under both
estimands.} Estimand (i): seed-averaged per-class coverage, then minimum over classes (used
throughout this paper). Estimand (ii): per-seed minimum over classes, then averaged over the
$10$ seeds, with standard deviation and per-seed range. $\alpha{=}0.10$.}
\label{tab:seed_dispersion}
\begin{tabular}{lccc}
\toprule
Method & Estimand (i) & Estimand (ii), mean $\pm$ sd & Per-seed range\\
\midrule
Split CP (baseline)                & 0.699 & $0.677\pm0.029$ & $[0.635,0.717]$\\
Source Mondrian (ours, label free) & 0.772 & $0.739\pm0.024$ & $[0.679,0.771]$\\
\bottomrule
\end{tabular}
\end{table}

\section{Stronger-backbone check (CTR-GCN)}
\label{supp:ctrgcn}

To confirm that the collapse and recovery pattern is not tied to ST-GCN, we repeat it with a stronger
feature extractor, a channel wise topology refinement GCN \citep{chen2021ctrgcn}, trained on the
same NTU-60 cross subject split (head top-1 $0.767$, above ST-GCN's $0.727$; tangent space
conformal backbone top-1 $0.675$, above ST-GCN's $0.627$; the two CTR-GCN figures and the ST-GCN
conformal figure come from released result files, while $0.727$ comes from project notes and
appears in none). This is a single joint stream network,
still below strong four stream ensembles ($\approx0.92$); the point is that the finding
\emph{persists as accuracy rises}, not a peak accuracy claim.

\paragraph{The finding reproduces on the SPD pipeline.}
Feeding CTR-GCN features through the same tangent space SPD conformal pipeline
(Table~\ref{tab:ctrgcn}), split CP again collapses per class ($0.673$ worst) at near nominal
marginal ($0.881$), and label free source Mondrian again recovers it ($0.721$, $+0.048$) while
holding marginal coverage on target: the identical qualitative pattern to the ST-GCN rows, at a
higher accuracy backbone. Weighted CP again buys worst class only by marginal over coverage.

\begin{table}[t]
\centering
\small
\caption{\textbf{[Real data, NTU-60 cross subject, CTR-GCN features] Recovery on a stronger backbone.}
Tangent-space conformal backbone on CTR-GCN-feature SPD (conformal top-1 $0.675$).
$\alpha{=}0.10$, $10$ seeds, $60$ classes. $^\circ$Threshold requires a labeled target pool.
$^\ast$Oracle needs target labels (ceiling).}
\label{tab:ctrgcn}
\begin{tabular}{lccccc}
\toprule
Method & Marg.\ cov. & Worst-class & $\%{<}0.85$ & $\%{<}0.80$ & Mean size\\
\midrule
Split CP (baseline)                & 0.881 & 0.673 & 32\% & 20\% & 2.98\\
Source Mondrian (ours, label free) & 0.880 & 0.721 & 20\% &  3\% & 3.77\\
Weighted CP                        & 0.910 & 0.735 & 20\% & 13\% & 4.01\\
Weighted class conditional         & 0.898 & 0.735 & 13\% &  3\% & 6.76\\
Margin abstention$^\circ$ ($89\%$ acc.) & 0.892 & 0.681 & 30\% & 20\% & 2.82\\
Target-oracle class cond.\ $^\ast$ & 0.908 & \textbf{0.899} &  0\% &  0\% & 4.48\\
\bottomrule
\end{tabular}
\end{table}

\paragraph{The collapse persists across backbones and heads.}
Conformalizing CTR-GCN's \emph{own} softmax head directly (LAC on its class probabilities, the
deployable single model recommendation) tells the same story: per class coverage collapses to
$0.558$ worst under split CP at $\alpha{=}0.10$ and source Mondrian recovers it to $0.677$
label free (and at $\alpha{=}0.01$, split worst $0.895\to$ Mondrian $0.932$). The mechanism is
visible in the \emph{intrinsically confusable} NTU actions, \emph{reading, writing,
play with phone, type on keyboard}, which stay at 42 to 56 percent per class accuracy even for
strong skeleton models, a pattern consistent with their near identical poses. That per class
accuracy range was transcribed from an original run log that is no longer available; the released
result file behind this table carries aggregate target top-1 accuracy and conformal metrics, and no
per class accuracy. Table~\ref{tab:ctrgcn_hard} shows these
classes remain badly under covered by split CP even at $0.767$ head accuracy, and source Mondrian
lifts each label free. The residual collapse thus persists across the tested backbones and heads,
consistent with data intrinsic class heterogeneity that a stronger backbone does not remove and
that class conditional calibration addresses directly.

\begin{table}[t]
\centering
\small
\caption{\textbf{[Real data, NTU-60 cross subject, CTR-GCN head] Hard-class slice.} Per class target
coverage for the four intrinsically confusable NTU actions, conformalizing CTR-GCN's own softmax
head (top-1 $0.767$). $\alpha{=}0.10$, $10$ seeds. Split CP undercovers them even at high
accuracy; source Mondrian recovers each label free.}
\label{tab:ctrgcn_hard}
\begin{tabular}{lccc}
\toprule
Hard class & Split CP & Source Mondrian & Oracle\\
\midrule
reading           & 0.558 & 0.815 & 0.906\\
writing           & 0.732 & 0.845 & 0.906\\
play with phone   & 0.719 & 0.834 & 0.915\\
type on keyboard  & 0.808 & 0.884 & 0.913\\
\bottomrule
\end{tabular}
\end{table}

\section{Generality beyond skeletons (CIFAR-100 under corruption shift)}
\label{supp:generality}

The collapse and recovery is not specific to skeleton data. We reproduce it on a completely
different modality, backbone, and shift type: \textbf{natural images} (CIFAR-100, $100$ classes),
a \textbf{CLIP ViT-L/14 zero shot} classifier \citep{radford2021clip} (no task training; one text
classifier scores both domains), and a \textbf{corruption shift} (Gaussian noise, source = clean,
target = corrupted). Source Mondrian calibrates on source labels only; target labels are used for
evaluation only, the same label free-on target protocol as our skeleton experiments.

The pattern is identical to NTU-60 (Table~\ref{tab:generality}): split CP holds near nominal
\emph{marginal} coverage ($0.916$) while \emph{per class} coverage collapses (worst class $0.601$;
$8\%$ of classes below $0.80$), and label free source Mondrian recovers it (worst class
$0.601\to0.784$, severely undercovered classes $8\%\to2\%$) while keeping marginal coverage on
target ($0.909$) and a
modest set size cost ($+1.01$). The recovery holds across the coverage regime: worst class
$0.387\to0.669$ at $\alpha{=}0.10$ and $0.910\to0.954$ at $\alpha{=}0.01$. That the same
marginal holds/per class collapses/label free-Mondrian-recovers structure appears on images with a
vision language backbone, far from skeletons and SPD geometry, indicates the phenomenon is a
property of class heterogeneous deployment shift in conformal prediction, not of the application.

\begin{table}[t]
\centering
\small
\caption{\textbf{[CIFAR-100, CLIP ViT-L/14 zero shot, corruption shift] Generality check.}
Source = clean, target = Gaussian-corrupted (target top-1 $0.651$). $\alpha{=}0.05$ (nominal
$0.95$), $10$ seeds, $100$ classes. Same collapse and recovery as the skeleton experiments, on a
different modality and backbone. $\ast$Oracle needs target labels (ceiling).}
\label{tab:generality}
\begin{tabular}{lccccc}
\toprule
Method & Marg.\ cov. & Worst-class & $\%{<}0.85$ & $\%{<}0.80$ & Mean size\\
\midrule
Split CP (baseline)                & 0.916 & 0.601 & 17\% & 8\% & 5.73\\
Source Mondrian (ours, label free) & 0.909 & 0.784 & 11\% & 2\% & 6.74\\
Target-oracle class cond.\ $^\ast$ & 0.964 & \textbf{0.931} & 0\% & 0\% & 12.41\\
\bottomrule
\end{tabular}
\end{table}

\subsection{A ten class replication (CIFAR-10 under the same shift)}
\label{supp:generality_k10}

Every benchmark above has many classes ($K{=}60$, $K{=}100$). To check that the phenomenon is not
an artifact of a large label space, we rerun the identical pipeline on CIFAR-10, holding the
backbone, the corruption family, the noise level, $\alpha$ and the seed protocol fixed
(Table~\ref{tab:generality_k10}). These are two different datasets, so the label space size is the
headline difference and not the only one; the difficulty gap is quantified below. The pattern
reproduces at $K{=}10$: split
CP holds marginal coverage at $0.909$ against nominal $0.95$ while the worst class falls to $0.778$
and one class of ten sits below $0.80$, and label free source Mondrian lifts the worst class to
$0.874$ with no class below $0.80$, holding marginal coverage at $0.908$.

Two features of the small $K$ regime deserve comment. First, the set size arithmetic is different:
mean set size is near $1$ throughout, because at ten classes with a $0.923$ accurate classifier a
set of the size seen at $K{=}100$ would name a large fraction of the label space. Recovery
therefore costs no additional set size here ($0.97$ to $0.96$), against $+1.01$ at $K{=}100$.
Second, mean set size alone understates the cost. The fraction of \emph{empty} prediction sets rises
from $4.1\%$ to $5.1\%$ under Mondrian, since per class thresholds tighten on easy classes as they
loosen on hard ones. The honest accounting is that Mondrian buys $+0.096$ worst class coverage and
removes the undercovered class for roughly one additional point of vacuous predictions.

We do \emph{not} read this pair as an isolation of the $\log K$ rate of the label complexity
theorem (main paper, Theorem~1). CIFAR-10 is also a substantially easier task than CIFAR-100 under
this corruption (target top-1 $0.923$ against $0.651$), so class count and problem difficulty move
together across these two points and a milder collapse is fully explained by either. The $K$
dependence rests on the theory; this experiment is a generality check across label space size, and
we report it as one.

\begin{table}[t]
\centering
\small
\caption{\textbf{[CIFAR-10, CLIP ViT-L/14 zero shot, corruption shift] Ten class replication.}
Identical backbone, corruption, noise level $\sigma{=}0.03$, $\alpha{=}0.05$ (nominal $0.95$) and
seed protocol as Table~\ref{tab:generality}, on a smaller label space and an easier task (target
top-1 $0.923$ against $0.651$; $10$ seeds, $10$ classes). ``Empty'' is the fraction of prediction sets containing no label.
$\ast$Oracle needs target labels (ceiling).}
\label{tab:generality_k10}
\begin{tabular}{lccccc}
\toprule
Method & Marg.\ cov. & Worst-class & $\%{<}0.80$ & Mean size & Empty\\
\midrule
Split CP (baseline)                & 0.909 & 0.778 & 10\% & 0.97 & 4.1\%\\
Source Mondrian (ours, label free) & 0.908 & 0.874 & 0\% & 0.96 & 5.1\%\\
Target-oracle class cond.\ $^\ast$ & 0.951 & \textbf{0.948} & 0\% & 1.10 & 0.7\%\\
\bottomrule
\end{tabular}
\end{table}

\clearpage

\section{What target labels buy: the measured label budget}
\label{supp:labelcurve}

\begin{figure}[!htbp]
\centering
\includegraphics[width=\linewidth]{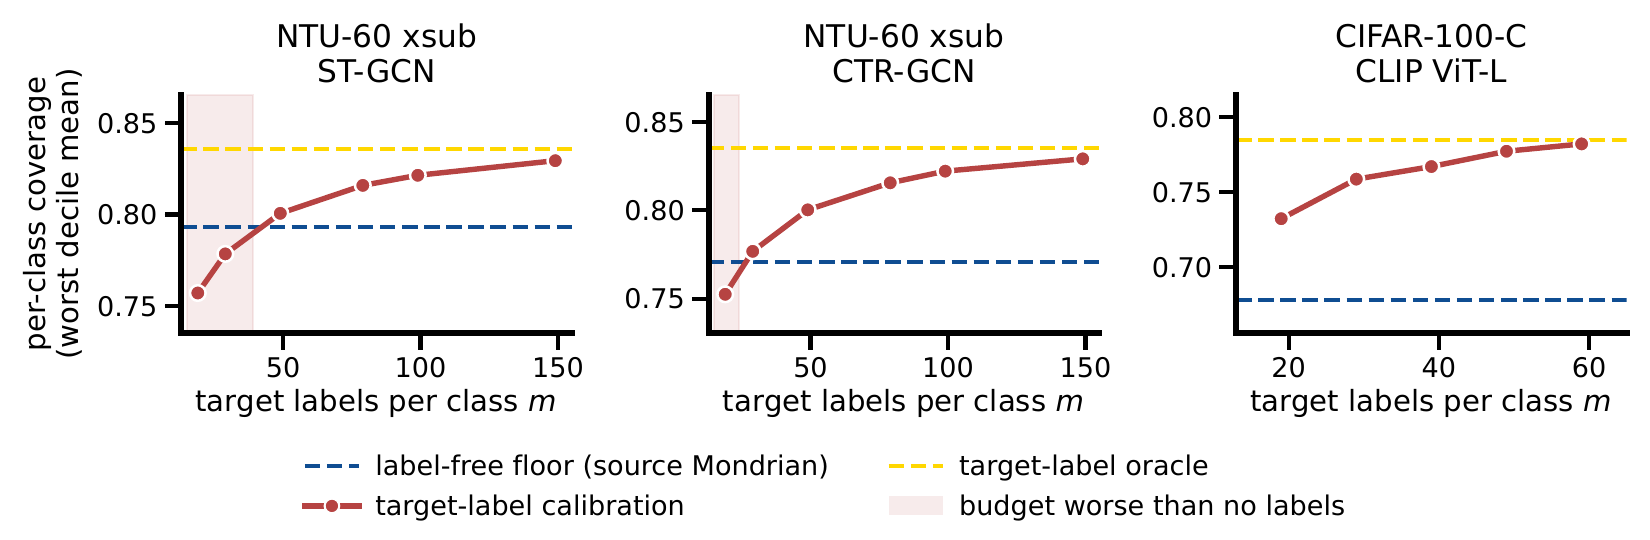}
\caption{\textbf{[Real data] What target labels buy.} Per class coverage
($\mathrm{CVaR}_{10}$, worst decile mean) against target labels per class $m$, at
$\alpha{=}0.10$ with $200$ resamples. Blue is the label free source Mondrian floor ($m{=}0$), gold
the target label oracle (full pool), red the audit-Mondrian curve. Shaded: budgets whose per class
coverage is \emph{below} the label free floor, so the labels are worse than useless. Those budgets
also inflate set size ($7.04$ against $4.61$ at $m{=}19$ on ST-GCN), so they are strictly dominated.
Crossings: $m\approx42$ and $m\approx26$ on NTU-60, and $m\le19$ on CIFAR-100-C, where the first
grid point is already above the floor and the value is an upper bound. The grid is rank aligned, so
the realized coverage level is nominal at every point.}
\label{fig:labelcurve}
\end{figure}

\paragraph{Setup.} The label complexity theorem (main paper, Theorem~1) is a statement about how
many labeled target draws per class are needed. Here we measure the corresponding curve directly.
Audit-Mondrian draws $m$ labeled target points per class from a pool held out from the evaluation
split, calibrates a per class threshold on them alone, and is scored on a fixed evaluation split
that is identical across all $m$, so the only quantity varying along the curve is the audit budget.
The $m{=}0$ endpoint is label free source Mondrian and the $m{=}\infty$ endpoint is the target label
oracle on the full pool. We report $200$ resamples at $\alpha{=}0.10$ on three settings: NTU-60
cross subject with ST-GCN and with CTR-GCN features, and CIFAR-100-C with the CLIP ViT-L/14 head.

Two protocol choices matter. First, the metric is $\mathrm{CVaR}_{10}$, the mean coverage of the
worst decile of classes. Worst class alone is a minimum over $60$ to $100$ classes on a finite
evaluation set and is dominated by the noise in that minimum, so it is unstable along a curve.
Second, the grid takes $m$ with $(m{+}1)(1{-}\alpha)$ integral. The split conformal threshold is the
$\lceil (m{+}1)(1{-}\alpha)\rceil$-th order statistic, so the realized level overshoots nominal by up
to $1/(m{+}1)$, and that overshoot is a deterministic sawtooth in $m$ that would otherwise ride on
top of the trend. On the aligned grid the realized level is nominal at every point (measured
$0.899$ to $0.901$ across all three panels), which makes the comparison across $m$ exact.

\paragraph{Finding: a small budget is worse than no budget.}
Figure~\ref{fig:labelcurve} shows the curve rising monotonically in $m$ across the budget grid
toward the oracle in all three settings. On NTU-60 that rise begins \emph{below} the label free
floor, so the curve does not start where spending no labels would put it. The informative part is
the left end. On NTU-60 the first grid points
fall \emph{below} the label free floor: with ST-GCN, $\mathrm{CVaR}_{10}$ is $0.757$ at $m{=}19$ and
$0.778$ at $m{=}29$ against a floor of $0.793$, and with CTR-GCN it is $0.752$ at $m{=}19$ against a
floor of $0.771$. These budgets are strictly dominated, because they also inflate the prediction
sets: mean set size at $m{=}19$ is $7.04$ against the floor's $4.61$ on ST-GCN and $5.87$ against
$3.41$ on CTR-GCN. Paying for a handful of target labels per class buys worse per class coverage and
larger sets than paying for none. The mechanism is variance: a per class quantile estimated from
$19$ points is noisy enough that the noise exceeds the bias of carrying the source quantile over.

Interpolating the crossing, target label calibration overtakes the label free floor at
$m\approx42$ (ST-GCN) and $m\approx26$ (CTR-GCN), and closes half the floor to oracle gap at
$m\approx76$ and $m\approx54$. On CIFAR-100-C the first usable grid point already sits above both
thresholds, so there we can only report an upper bound of $m\le19$ for each.

\paragraph{Scope: this measures a label budget.} Two limits are worth stating.
The $\log K$ dependence is not isolated here: CIFAR-100-C at $K{=}100$ needs \emph{fewer} labels than
NTU-60 at $K{=}60$, the opposite of what a naive reading of the rate would suggest, because the
dominant factor is how close the label free floor already sits to the oracle. The floor to oracle
gap is $0.042$, $0.065$ and $0.107$ across the three panels, and the settings with the least room
need the most labels to claim it. One $\alpha$ and two values of $K$ cannot separate class count
from that effect.

The second limit concerns which guarantee fails at small $m$. Marginal validity does \emph{not}
collapse: mean per class coverage sits at nominal at every grid point, including the points that
fall below the floor. What a small audit fails to buy is \emph{uniform} per class validity, since
the variance of the per class thresholds spreads coverage across classes even while its average is
correct. That is exactly the separation Theorem~1 draws between validity alone, which needs few
labels, and validity together with efficiency, which does not.

\section{Pseudo-label efficiency ceiling: prediction powered per class calibration}
\label{supp:ppi}

\paragraph{Setup.} The label complexity theorem (main paper) is a minimax statement: it treats
a labeled audit set as the only source of information about $P_T(Y\mid X)$ and shows unlabeled target
data cannot improve the rate at which it recovers per class coverage. In practice, however, the
classifier under evaluation also supplies free pseudo labels on the unlabeled target pool, and
PPI~\citep{angelopoulos2023ppi} is designed to exploit exactly this
kind of correlated, cheap surrogate to debias an estimate using a small number of true labels. We
test PPI as an alternative to Audit-Mondrian (main paper, label complexity section) for estimating the
per class conformal quantile $q_c^\star$ at a fixed total labeled budget $M$ split across classes, on
two real backbone/dataset pairs: NTU-60 cross subject with a CTR-GCN softmax head
\citep{chen2021ctrgcn} (Section~\ref{supp:ctrgcn}), and CIFAR-100 under corruption shift with CLIP
zero shot \citep{radford2021clip}. The CIFAR pair here is a \emph{different and much harder} CLIP
configuration than the generality check of Section~\ref{supp:generality}: it uses ViT-B/32 at
corruption level $\sigma{=}0.08$, where target top-1 is $0.264$ and split conformal reaches only
$0.476$ marginal coverage against nominal $0.90$, against ViT-L/14 at $\sigma{=}0.03$ with target
top-1 $0.651$ and marginal coverage $0.916$ there. The two must not be read as the same setting.
This places the CIFAR column of the PPI analysis in the severe shift regime, where marginal
coverage has itself collapsed, so its ceiling should be read as evidence about that regime and the
NTU-60 column carries the mild regime. Rerunning the PPI ceiling on the ViT-L/14 cache would place
both columns in the same regime and is left to future work.

\paragraph{Naive vs.\ PPI audit at matched budget.} The naive audit uses only the $m_c$ true labels
per class (Audit-Mondrian). The PPI audit additionally uses the unlabeled pseudo labelled pool: it
forms the per class quantile estimate as the naive audit estimate minus $\lambda$ times (the
pseudo label estimate on the audit indices minus the pseudo label estimate on the full unlabeled
pool), for a tuning parameter $\lambda$, with $\lambda{=}1$ the standard, untuned, deployable choice
\citep{angelopoulos2023ppi}. We validate every configuration with a two layer guard: (i) an aggregate
check, does the resulting worst class / \%$<$0.80 summary get worse, and (ii) a same class
check, does PPI newly break per class validity on a class the naive audit kept valid at the identical
budget. Both layers flag harm below.

\paragraph{The untuned estimator harms.} At every labeled budget we test, $\lambda{=}1$ PPI is worse
than the naive audit alone. On NTU-60 CTR-GCN, at total budget $M{=}300$ the worst decile per class
coverage (the mean over the lowest ten percent of per class coverages, denoted cvar10) is $0.477$
for PPI vs.\ $0.737$ for naive; PPI newly breaks per class validity (undoes
coverage the naive audit had achieved) on $39$ classes ($4$ of them the intrinsically hard classes of
Table~\ref{tab:ctrgcn_hard}) at $M{=}300$, and still on $15$ classes ($2$ hard) at $M{=}600$. The
measured per class quantile variance reduction ratio (median over classes, naive audit variance over
PPI variance) is $0.45\times$ on NTU-60, i.e.\ PPI \emph{increases} variance and does not reduce
it, with Spearman correlation between this (harmful) ratio and classifier accuracy $1{-}\rho$ of
$0.83$. On CIFAR-100-C/CLIP the same pattern holds: variance ratio $0.48\times$, Spearman $-0.59$,
and PPI breaks per class validity at every budget we test, up to $M{=}4000$. Both failures are caught
by our validity guard before any downstream use, this is why we do not recommend $\lambda{=}1$ PPI
as a method, and why we instead ask what the best possible tuning could achieve.

\paragraph{The oracle ceiling: is the harm fixable by tuning $\lambda$?} The $\lambda{=}1$ harm could
in principle be a tuning artifact and not a structural limit. We therefore compute the best case
directly: the oracle $2$-D PPI++ label efficiency gain is $\mathrm{gain}=1/(1-R^2)$, where $R^2$ is the
squared multiple correlation of the naive per class quantile influence function with the $2$-D span of
pseudo label control variates (the pseudo label indicator $\mathbf{1}\{\hat y=c\}$ and the thresholded
interaction $\mathbf{1}\{s(X,c)\le q_c^\star,\ \hat y=c\}$), evaluated at the oracle optimal $\lambda$, an unbounded unlabeled pool, and the true
target quantile. This is the standard PPI++ efficiency identity \citep{angelopoulos2023ppipp}
specialized to a scalar per class quantile target; $\mathrm{gain}\ge1$ always, with equality when the
pseudo label carries no information ($R^2\to0$). Because it assumes oracle tuning, an infinite
unlabeled pool, and the (unknown, in deployment) true quantile, it is an asymptotic best case for
this control span; a finite sample, tunable-$\lambda$ estimator should not be expected to
systematically exceed it, so the reported ceiling is, if anything, favorable to PPI, making the
negative reading below conservative and never overstated. We certify every reported number: $0$ classes are non finite or skipped, and
$\mathrm{gain}_{\mathrm{multi}}\ge\mathrm{gain}_{\mathrm{scalar}}$ holds for every class on both
datasets (Table~\ref{tab:ppi_oracle}).

\begin{table}[t]
\centering
\small
\caption{\textbf{Real data. Oracle $2$-D PPI++ label efficiency ceiling, per dataset.} Best case: oracle
$\lambda$, infinite unlabeled pool, true target quantile; not a deployable estimator. ``Collapsing''
classes are those where the label free source Mondrian floor already undercovers (per class
coverage $<0.80$ at $m{=}0$), which is the subset the estimator is being asked to repair.
$\alpha{=}0.10$. The CIFAR column is the
CLIP ViT-B/32 $\sigma{=}0.08$ configuration (target top-1 $0.264$), a severe shift regime, and is
\emph{not} the ViT-L/14 generality setting of Table~\ref{tab:generality}.}
\label{tab:ppi_oracle}
\begin{tabular}{lcc}
\toprule
Metric & NTU-60 CTR-GCN & CIFAR-100-C / CLIP\\
\midrule
$K$ (classes)                                  & 60    & 100\\
$\bar\rho$ (mean pseudo label disagreement)    & 0.235 & 0.734\\
All classes: median gain                       & $1.07\times$ & $1.01\times$\\
All classes: max gain                          & $3.36\times$ & $1.06\times$\\
All classes: \% gain $\ge3\times$              & 2\%   & 0\%\\
Spearman(gain, $1{-}\rho$), all classes        & 0.96  & 0.79\\
Collapsing classes: $n$                        & 8     & 97\\
Collapsing classes: median gain                & $1.05\times$ & $1.01\times$\\
Collapsing classes: max gain                   & $1.08\times$ & $1.06\times$\\
\bottomrule
\end{tabular}
\end{table}

\paragraph{Mechanism.} On both datasets, gain tracks classifier accuracy closely (Table~\ref{tab:ppi_oracle}):
the pseudo label is a more informative control variate exactly where the classifier already agrees
with the truth. Shift breaks this precisely on the classes whose per class coverage collapses, it
decorrelates the pseudo label from the ground truth on those classes, so the $2$-D control span the
estimator relies on carries almost no signal ($R^2\to0$) where efficiency is needed most; the
harder shifted CIFAR-100-C/CLIP ViT-B/32 setting has both a higher mean disagreement
($\bar\rho{=}0.734$ vs.\ $0.235$) and a uniformly lower ceiling than NTU-60. The intrinsically confusable NTU actions
(Table~\ref{tab:ctrgcn_hard}) illustrate this at the individual class level: reading ($\rho{=}0.71$)
caps at $1.01\times$ and writing ($\rho{=}0.68$) at $1.02\times$, while play with phone
($\rho{=}0.45$) and type on keyboard ($\rho{=}0.41$) reach $1.03\times$.

\paragraph{Reading.} Two independent lines of evidence agree: the untuned, deployable PPI estimator
actively harms, and the idealized, non deployable oracle ceiling shows this is not fixable by better
tuning, on the classes where per class coverage collapses, no amount of $\lambda$-tuning or pool
size manufactures efficiency the pseudo label does not carry. The result is an empirical measurement
complementing, not superseding, the label complexity theorem (main paper): the theorem shows unlabeled data
cannot help in the worst case over all consistent target laws; this experiment shows that, on two
real shifts and two modalities, the single most favorable use of unlabeled data available in
practice, the classifier's own pseudo labels, does not help either, exactly where it would matter.

\section{\texorpdfstring{Coverage-level ($\alpha$) sweep}{Coverage-level alpha sweep}}
\label{supp:alpha_sweep}

To test whether the per class collapse is an artifact of the single operating point $\alpha{=}0.10$,
we sweep $\alpha\in\{0.05,0.10,0.15,0.20\}$ on the same NTU-60 xsub ST-GCN (full) cache, no
retraining, $10$ seeds. Table~\ref{tab:alpha_sweep} reports worst class per class coverage.

\begin{table}[t]
\centering
\small
\caption{\textbf{[Real data, NTU-60 cross subject] $\alpha$-sweep, worst class per class coverage.}
Same cache and protocol as Table~\ref{tab:recovery}; mean over $10$ seeds, $60$ classes.
$^\ast$Oracle calibrates on target labels (not deployable; the ceiling).}
\label{tab:alpha_sweep}
\begin{tabular}{lcccccc}
\toprule
$\alpha$ & Nominal & Split CP & Source-CC & Weighted CP & wCC & Oracle$^\ast$\\
\midrule
0.05 & 0.95 & 0.824 & 0.840 & 0.913 & 0.857 & 0.949\\
0.10 & 0.90 & 0.699 & 0.772 & 0.803 & 0.809 & 0.890\\
0.15 & 0.85 & 0.544 & 0.706 & 0.687 & 0.740 & 0.843\\
0.20 & 0.80 & 0.427 & 0.662 & 0.537 & 0.708 & 0.789\\
\bottomrule
\end{tabular}
\end{table}

\paragraph{Finding.}
The collapse is not specific to $\alpha{=}0.10$: the split CP worst class to nominal gap grows
monotonically from $0.13$ ($\alpha{=}0.05$) to $0.37$ ($\alpha{=}0.20$). Label free source Mondrian
raises the worst class at every level, by $+0.02$, $+0.07$, $+0.16$, $+0.24$ as $\alpha$ increases,
i.e.\ by more where the collapse is more severe, while its marginal coverage tracks split CP's
(both slightly below nominal: source $0.939/0.881/0.825/0.772$ across the four levels). Weighted CP
reaches higher worst class but only through marginal over coverage throughout (marginal
$0.975/0.928/0.876/0.822$ vs.\ nominal). The headline pattern is thus robust across the coverage
regime.

\section{Cross-view shift (NTU-60 cross-view): full method breakdown}
\label{supp:crossview}

The main paper summarizes the mild cross-view shift; the full six method breakdown is in
Table~\ref{tab:xview}.

\begin{table}[t]
\centering
\small
\caption{\textbf{[Real data, NTU-60 cross-view] Recovery under a mild cross-view shift.} Six
methods, 10 seeds, ST-GCN tangent backbone, nominal 0.90. Marginal coverage is above nominal
yet the worst class stays below it; source Mondrian recovers label free at a small set-size
cost. $^\dagger$On this mild shift margin abstention's CRC threshold accepts every point
(accept rate $1.0$), so it reduces to Split-CP.}
\label{tab:xview}
\begin{tabular}{lcccc}
\toprule
Method & Marginal cov. & Worst-class cov. & Mean set size & Classes ${<}0.80$ (of 60)\\
\midrule
Split-CP              & 0.924 & 0.803 & 4.17  & 0\\
Source Mondrian       & 0.928 & 0.875 & 5.21  & 0\\
Weighted CP           & 0.948 & 0.870 & 5.83  & 0\\
Weighted CC           & 0.937 & 0.870 & 13.06 & 0\\
Margin abst.$^\dagger$ & 0.924 & 0.803 & 4.17  & 0\\
\textbf{Oracle}       & \textbf{0.906} & \textbf{0.893} & \textbf{4.01} & \textbf{0}\\
\bottomrule
\end{tabular}
\end{table}

\section{\texorpdfstring{Cross-dataset shift (NTU\,$\to$\,N-UCLA): full method breakdown}{Cross-dataset shift (NTU to N-UCLA): full method breakdown}}
\label{supp:crossdataset}

The main paper summarizes this cross sensor result; the full six method breakdown is in
Table~\ref{tab:crossdataset}.

\begin{table}[t]
\centering
\small
\caption{\textbf{[Real data, NTU-60\,$\to$\,N-UCLA cross dataset] Recovery under a cross sensor shift.}
$\alpha{=}0.10$, $10$ seeds, five shared classes, target top-1 $0.598$. $\ast$Oracle needs target
labels (ceiling). $\dagger$Margin abstention's CRC threshold also needs a labeled target pool.}
\label{tab:crossdataset}
\begin{tabular}{lccc}
\toprule
Method & Marg.\ cov. & Worst-class & Mean size\\
\midrule
Split CP (baseline)                        & 0.501 & 0.000 & 0.72\\
Source Mondrian (ours, label free)         & 0.494 & 0.001 & 0.75\\
Weighted CP                                & 0.968 & \textbf{0.837} & 4.57\\
Weighted class conditional                 & 0.864 & 0.750 & 3.55\\
Margin abstention$^\dagger$                 & 0.358 & 0.000 & 0.59\\
Target-oracle class cond.\ $^\ast$          & 0.913 & \textbf{0.907} & 2.48\\
\bottomrule
\end{tabular}
\end{table}

\paragraph{The geometry aware candidate's diagnostic.}
A geometry aware label free candidate, which reweights per class quantiles by log Euclidean
geodesic proximity to the target class means, also undercovers on this shift. It is one of the
source only, label free methods the main text reports as failing to recover here. The diagnostic
behind that failure is as follows. Its importance weights keep an
effective sample size of at least 68 percent of the calibration points on every class, so the
weights themselves stay unconcentrated. Even so, its reweighted per class source quantiles, which
range from 0.01 to 0.82 across classes, fall short of every target class threshold, which ranges
from 0.78 to 1.00, by amounts between 0.18 and 0.97. Source true class scores are concentrated too
low relative to the target, the support gap the main paper's impossibility result describes. The
released result files carry neither this candidate's effective sample sizes nor its per class
quantiles. These diagnostic figures were transcribed from original run output that is no longer
available, so they cannot be independently verified or recomputed from the released artifacts.
\section{Synthetic Controlled Study: Full Details}
\label{app:synthetic}

\emph{All numbers and figures in this appendix are from a controlled synthetic SPD shift.
They are mechanism illustrations only and should not be read as real data evidence.}

The synthetic study uses a class conditional SPD generator: $K{=}5$ classes, $250$ descriptors
per class, $d{=}6$, in a \emph{graded} regime (within class spread $=$ shift strength $=0.3$).
We fix $\alpha{=}0.10$ and report two disjoint seed ranges (primary $0$--$9$, held out
$100$--$109$) as mean$\pm$std. No hyperparameter is tuned to the outcome.

\subsection*{H1: Split CP undercovers (SYNTHETIC)}
\label{app:h1}
A source calibrated split CP threshold holds at nominal in distribution (source coverage
$0.896/0.907$) but undercovers the shifted target, dropping to $0.735/0.791$
(Figure~\ref{fig:coverage}, Table~\ref{tab:coverage}).
The shift is detectable, min distance AUROC $0.900/0.884$, yet detectability does not buy
safety: at $50\%$ acceptance, selective coverage is only $0.757/0.825$, below nominal.
This is the ``high OOD-AUROC $\ne$ safe selective classification'' phenomenon \citep{severeshift2026}
reproduced under a coverage lens.

\subsection*{H2: Geodesic score tightens in distribution sets (SYNTHETIC)}
\label{app:h2}
For reference: a \emph{geodesic nonconformity score} $\sig(x,c)=\dLE(\varphi(x),\Mc)$
(different from the LAC score used in the main results) yields tighter in distribution prediction
sets than a Euclidean prototype score: $1.54/1.52$ classes vs.\ $3.83/3.75$ at matched
${\approx}0.90$ coverage, that is $2.30/2.23$ classes smaller (Figure~\ref{fig:h2},
Figure~\ref{fig:h2size}). The geodesic score gives sets $0.54/0.50$ classes \emph{larger} than LAC
($1.00/1.02$), which exploits softmax sharpness on this low temperature backbone, a different
mechanism. This result supports geodesic geometry for SPD but is not load bearing.

\begin{figure}[tbp]
\centering
\includegraphics[width=\linewidth]{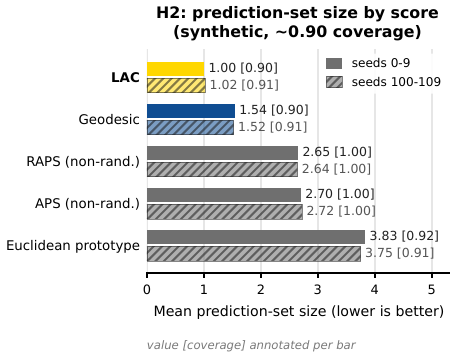}
\caption{\textbf{Synthetic study. H2: mean prediction set size} at ${\approx}0.90$ coverage, $5$ classes (lower is better). Seeds $0$--$9$ (solid) and $100$--$109$ (hatched); coverage in brackets. Synthetic setting: $K{=}5$, $250$/class, $d{=}6$, in distribution (shift strength $0$).}
\label{fig:h2size}
\end{figure}

\begin{figure}[tbp]
\centering
\includegraphics[width=\linewidth]{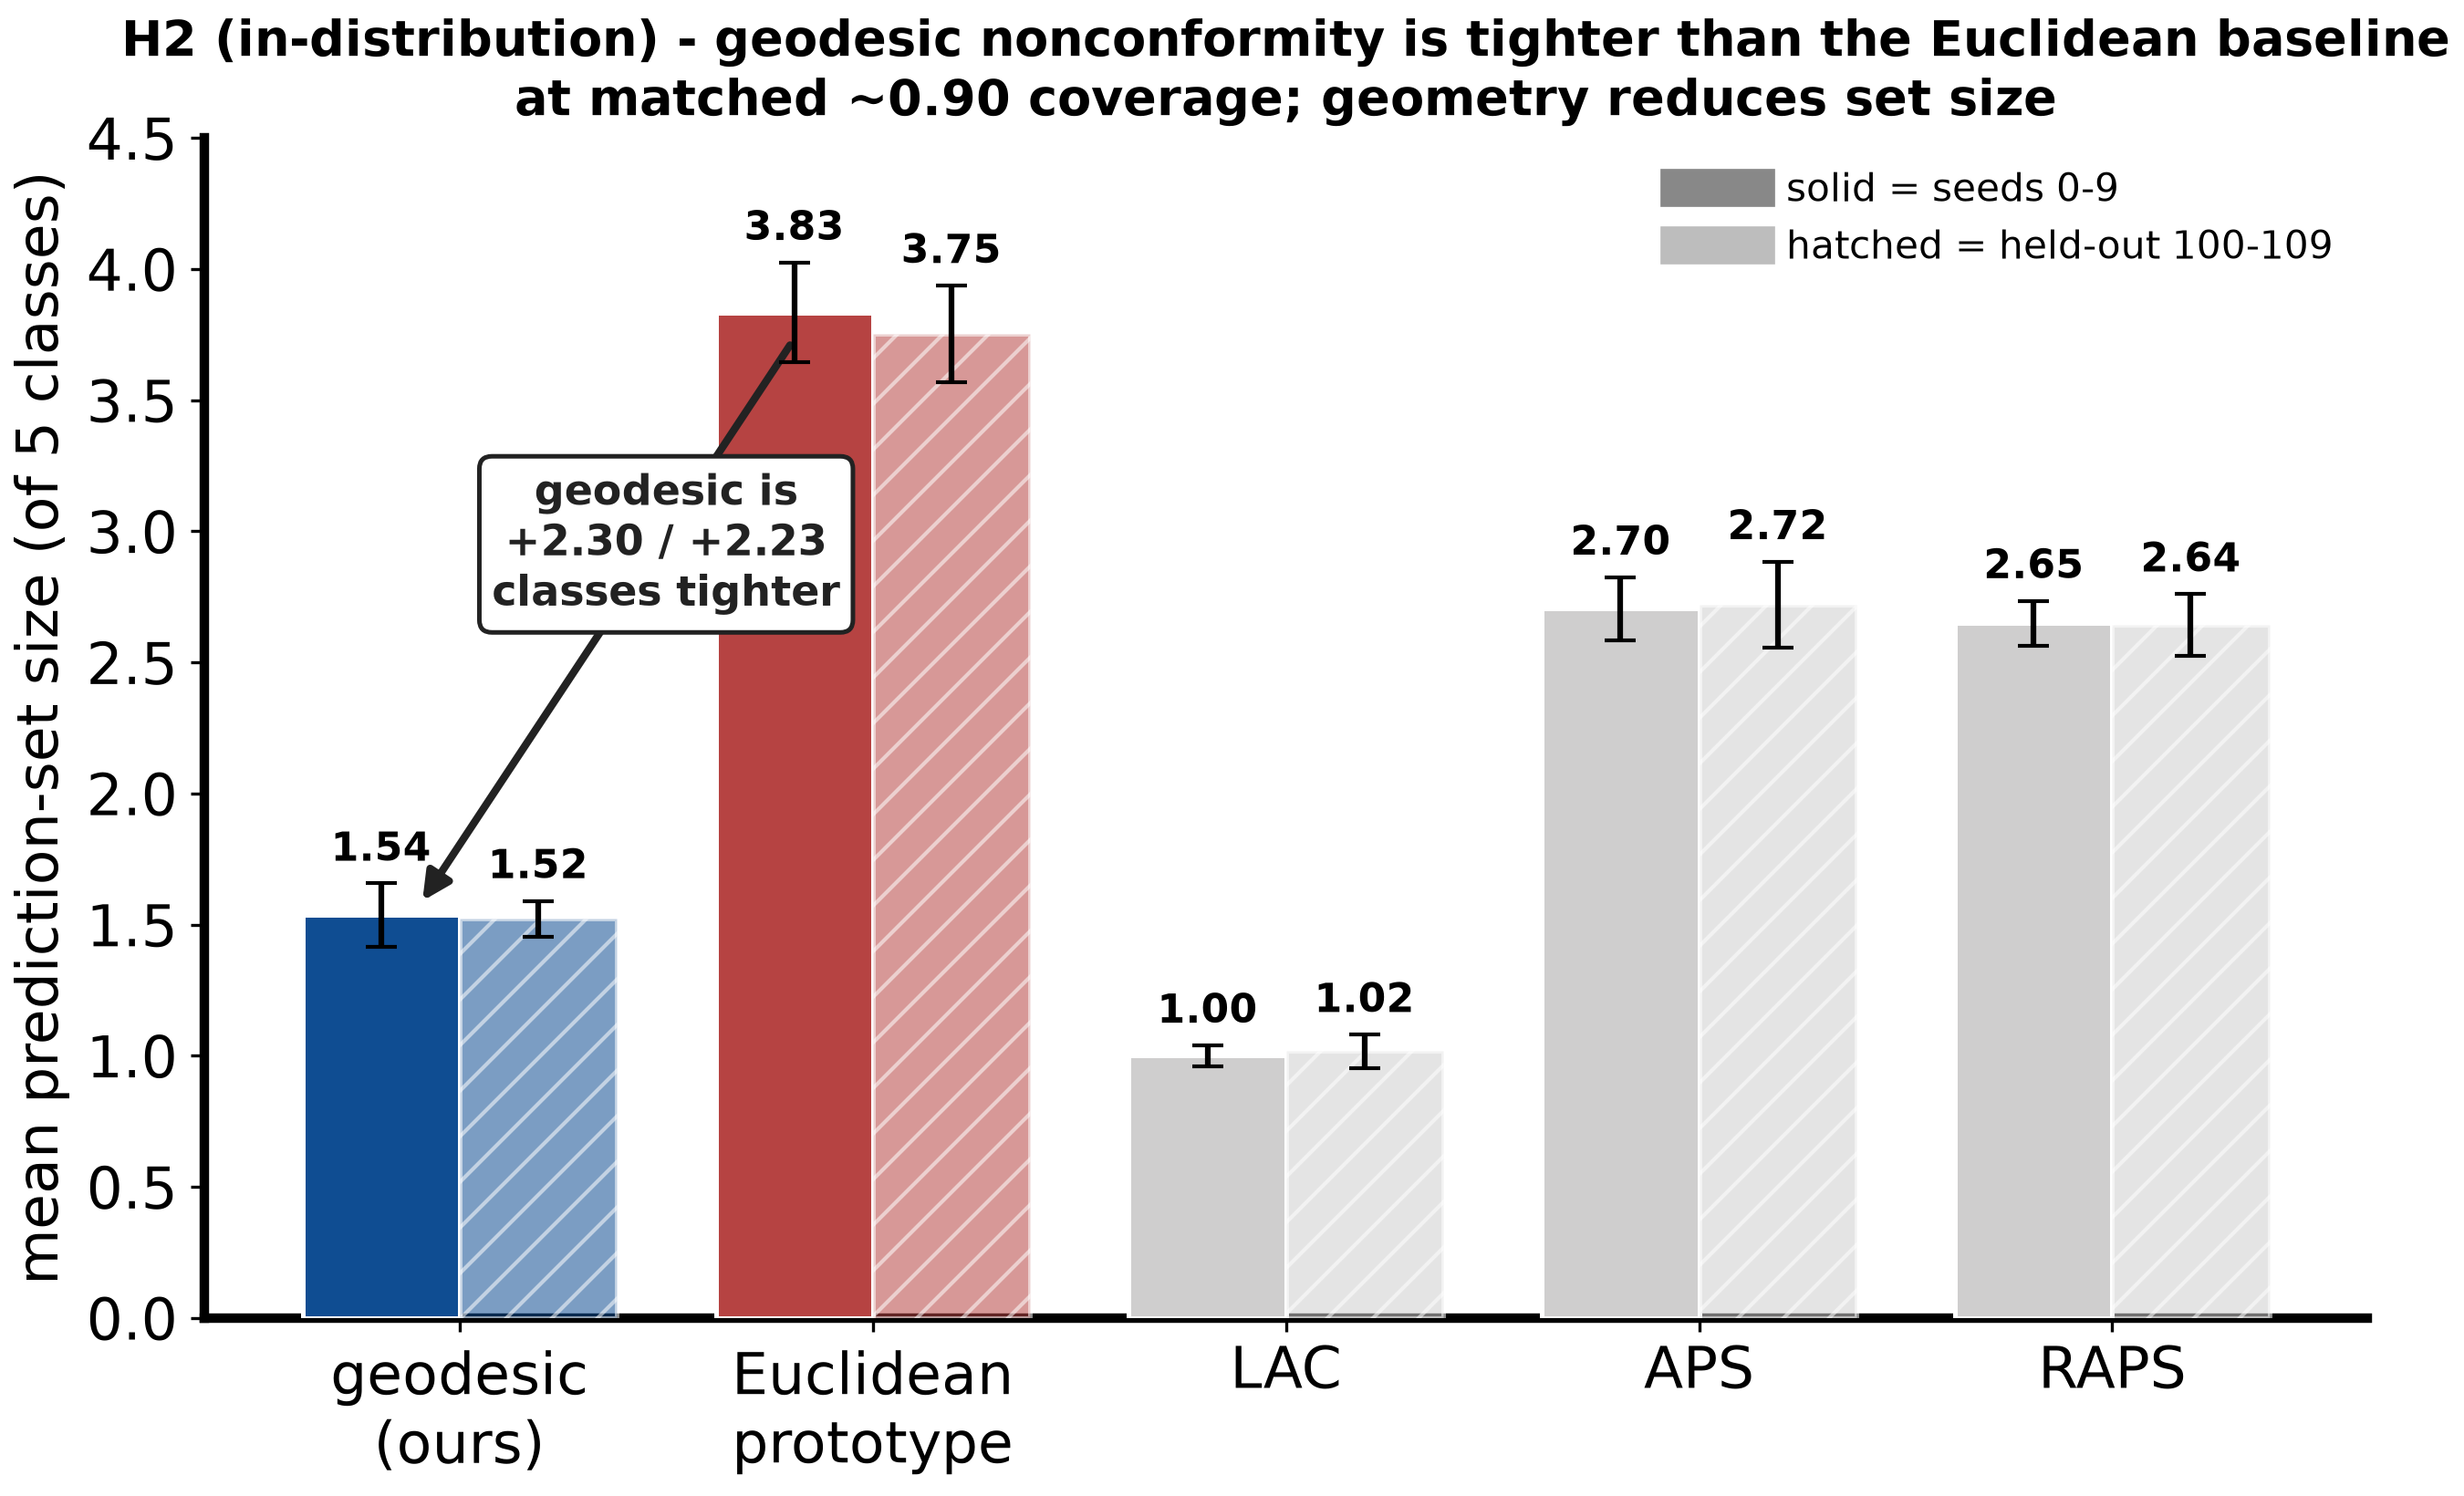}
\caption{\textbf{Synthetic study. H2: geodesic vs.\ flat nonconformity scores, in distribution.}
Averaged over the two seed ranges, geodesic sets are $2.26$ classes smaller than the Euclidean
prototype; LAC (smallest, using softmax sharpness) is $0.52$ classes smaller than geodesic. Seeds
$0$--$9$ solid, $100$--$109$ hatched.
Synthetic setting: $K{=}5$, $d{=}6$, shift $0$.}
\label{fig:h2}
\end{figure}

\subsection*{H3: Weighted CP restores marginal coverage, at a cost (SYNTHETIC)}
\label{app:h3}
Weighted exact CP restores marginal target coverage from $0.735/0.791$ to $0.956/0.944$ but
inflates sets ${\approx}4\times$ (Table~\ref{tab:coverage}, Figure~\ref{fig:coverage}).
The marginal recipe does not recover ($0.704/0.729$). This illustrates why, on the real benchmark,
weighted CP recovers marginal coverage while recovering per class coverage only inefficiently.

\begin{table}[tbp]
\centering
\small
\caption{\textbf{Synthetic study. H1/H3 coverage and size under shift} (nominal $0.90$). Source
split CP holds in distribution; target split CP undercovers; weighted exact restores marginal
coverage but inflates sets ${\approx}4\times$. Mean over seeds $0$--$9$ / $100$--$109$.
Synthetic setting: $K{=}5$, $250$/class, $d{=}6$, shift $0.3$.}
\label{tab:coverage}
\begin{tabular}{lcc}
\toprule
Method & Target coverage & Mean size\\
\midrule
Source split CP (in distribution) & 0.896 / 0.907 & -- \\
Target split CP (H1) & 0.735 / 0.791 & 0.86 / 0.90\\
Weighted marginal & 0.704 / 0.729 & 0.86 / 0.84\\
\textbf{Weighted exact (H3)} & \textbf{0.956 / 0.944} & 3.63 / 3.80\\
\bottomrule
\end{tabular}
\end{table}

\begin{figure}[tbp]
\centering
\includegraphics[width=\linewidth]{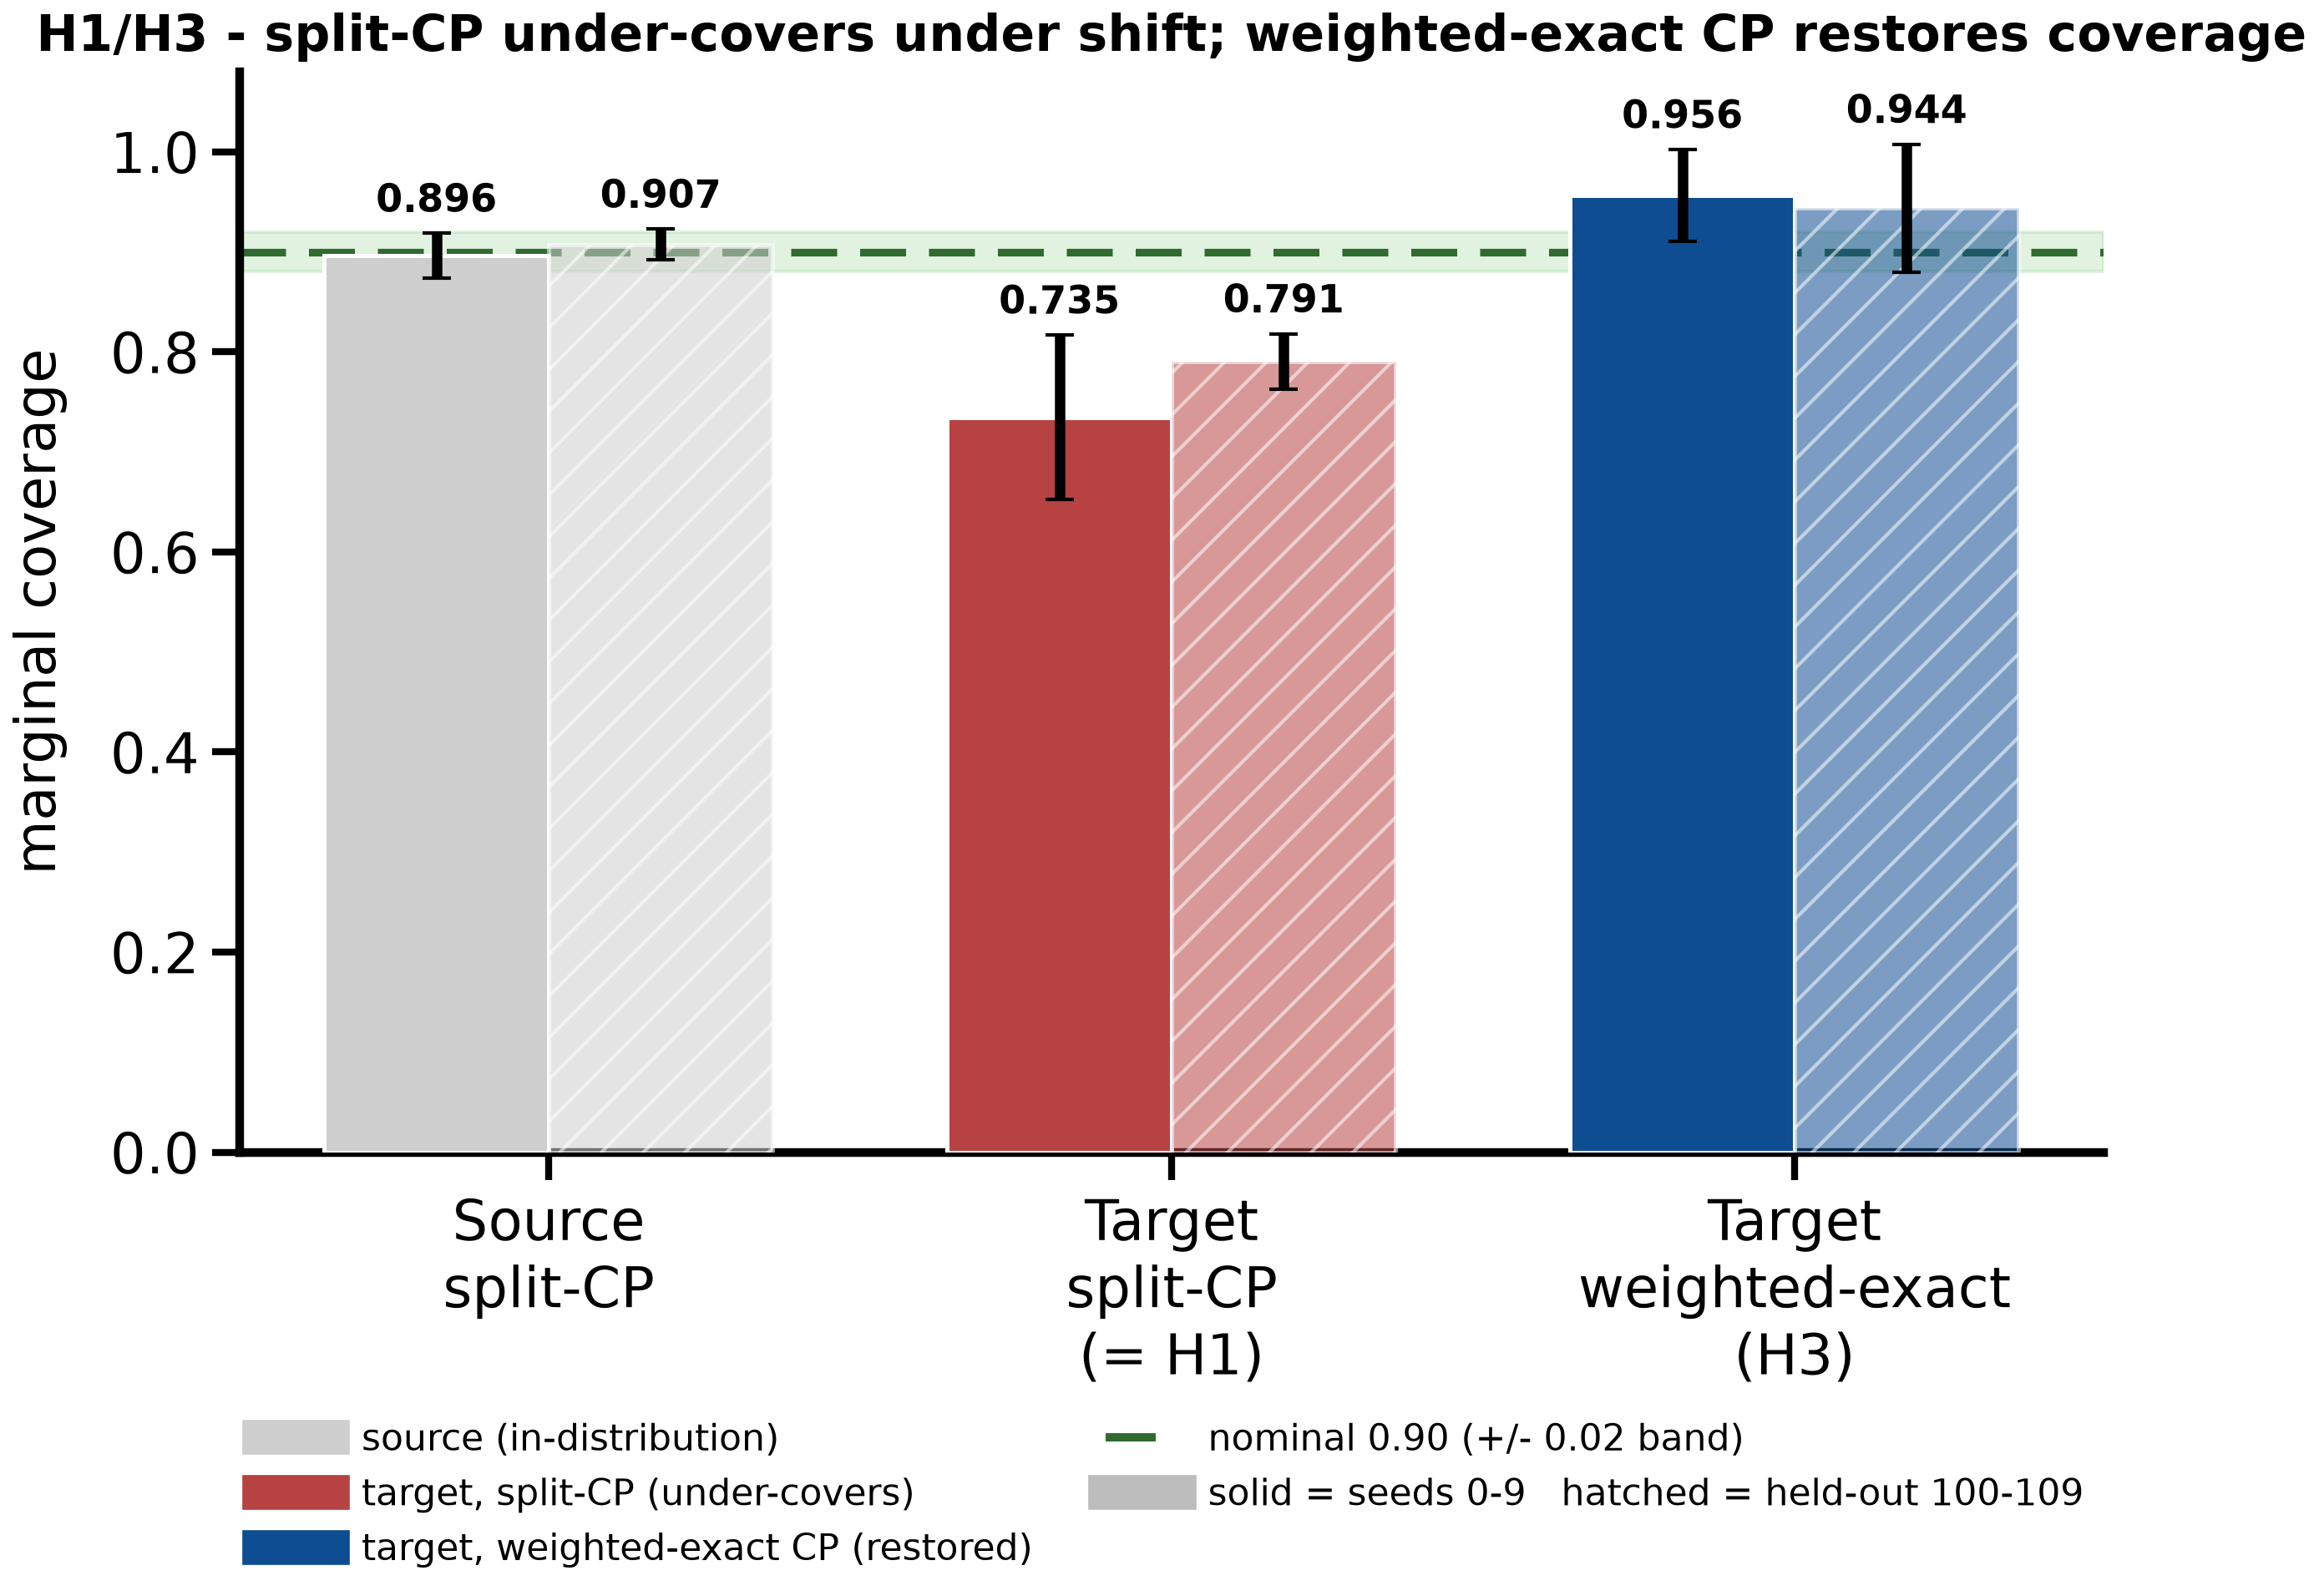}
\caption{\textbf{Synthetic study. H1/H3 marginal coverage recovery.} Split CP undercovers target;
weighted exact restores nominal. Solid $=$ seeds $0$--$9$, hatched $=$ $100$--$109$.
Synthetic setting: $K{=}5$, $d{=}6$, shift $0.3$.}
\label{fig:coverage}
\end{figure}

\subsection*{H4: Margin abstention, negative control (SYNTHETIC)}
\label{app:h4}

\emph{H4 is a negative control: even given a labeled target pool to calibrate the abstention
threshold, margin abstention does not address per class undercoverage.}

\paragraph{The signal dichotomy on the synthetic shift.}
Figure~\ref{fig:concept} lays out the resulting pipeline. The min distance OOD score has high
source versus target AUROC ($0.898/0.881$) but miscoverage AUROC of only $0.549/0.574$: it ranks
distributional outliers while missing miscovered points. The geodesic margin has low source versus target AUROC
($0.576/0.593$) but miscoverage AUROC $0.895/0.894$: on this synthetic shift, miscovered points
are pushed toward the wrong class mean (small min distance) but look ambiguous (small margin), so
the margin ranks miscovered points better (Figure~\ref{fig:dichotomy}). Figure~\ref{fig:manifold}
renders the same mechanism as geometry on the SPD manifold.

\begin{figure}[tbp]
\centering
\includegraphics[width=\linewidth,height=0.72\textheight,keepaspectratio]{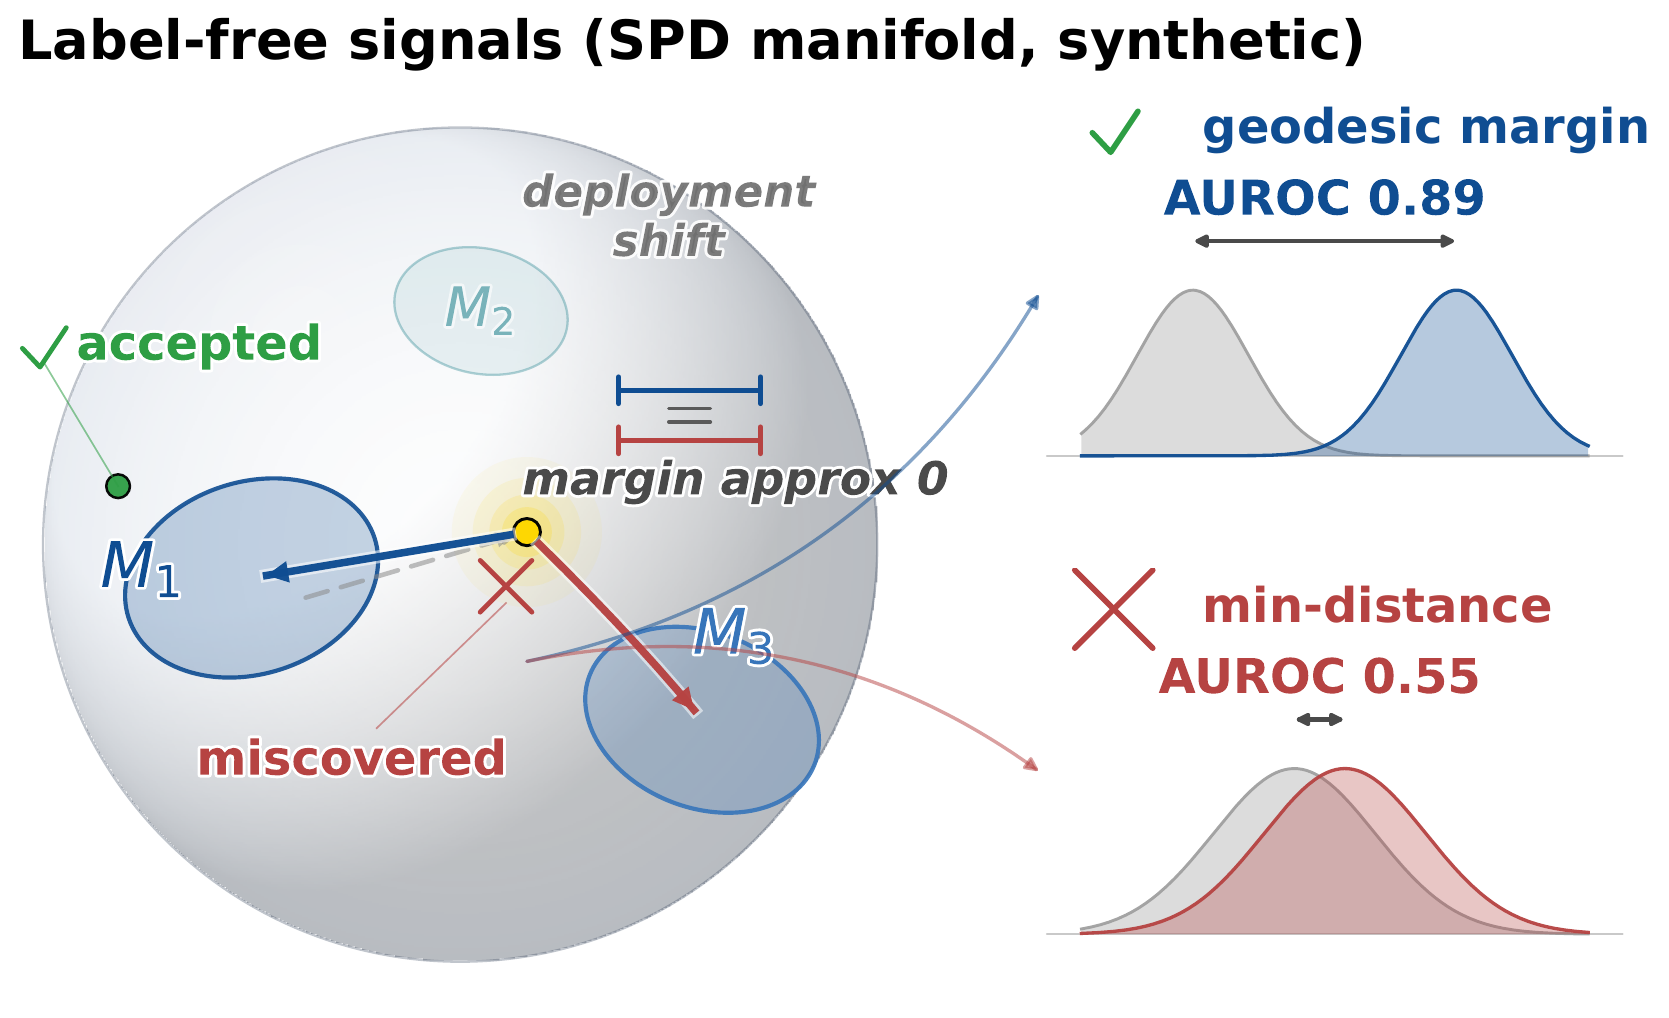}
\caption{\textbf{Synthetic schematic. Label free signals on the SPD manifold.} A target point drifts
under deployment shift toward the wrong class mean $M_3$. The min distance signal sees a short
geodesic to $M_3$ and calls the point in support (the trap; miscoverage AUROC $0.55$), while the
geodesic margin notices $d(x,M_1)\approx d(x,M_3)$ and flags it (miscoverage AUROC $0.89$). The
lower strips sketch the resulting score separation. The geometry is illustrative; the two AUROC
numbers are the measured synthetic values reported above.}
\label{fig:manifold}
\end{figure}

\begin{figure}[tbp]
\centering
\includegraphics[width=\linewidth,height=0.62\textheight,keepaspectratio]{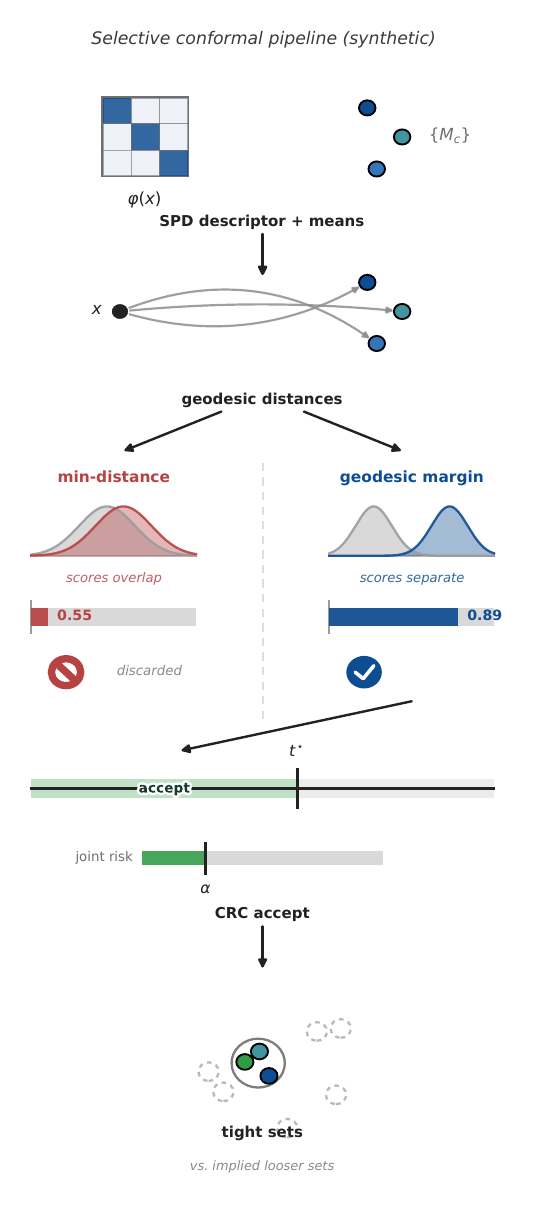}
\caption{\textbf{Synthetic study. Selective conformal pipeline.} Geodesic distances to the class means yield two label free signals; the min distance OOD signal ranks distributional outliers and is discarded, while the geodesic margin ranks miscoverage and is kept, then thresholded by CRC to accept a region with tight source calibrated sets. Synthetic setting: $K{=}5$, shift $0.3$.}
\label{fig:concept}
\end{figure}

\paragraph{The CRC operating point (requires labeled target pool).}
Setting the threshold by CRC \eqref{eq:crc} (using a labeled target pool) accepts $75\%/82\%$
of points, at conditional accepted coverage $0.869/0.885$ ($<$ nominal; only the joint marginal
risk is controlled, a weaker guarantee than conditional coverage) and accepted set size $0.948/0.961$ , 
$3.82\times/3.96\times$ tighter than weighted exact's $3.63/3.80$
(Figure~\ref{fig:h4crc}; Figures~\ref{fig:efficiency},~\ref{fig:crc}). Joint risk mean $0.097/0.095\le\alpha{+}0.01$,
per seed max $0.130/0.125$ (only the mean is guaranteed).

\paragraph{Synthetic H4 limitations.}
The geodesic margin's miscoverage AUROC ($0.89$) is comparable to a softmax confidence baseline
($0.95/0.96$) and does not exceed it; its value is being geometry aware at the softmax level. The OOD-trap / margin
contrast is shown on one synthetic shift family; class specific shifts and real backbones are
untested. On the real NTU-60 benchmark, margin abstention does not reduce per class undercoverage
even with this favorable synthetic shift mechanism operating (Table~\ref{tab:recovery}).

\begin{figure}[tbp]
\centering
\includegraphics[width=\linewidth]{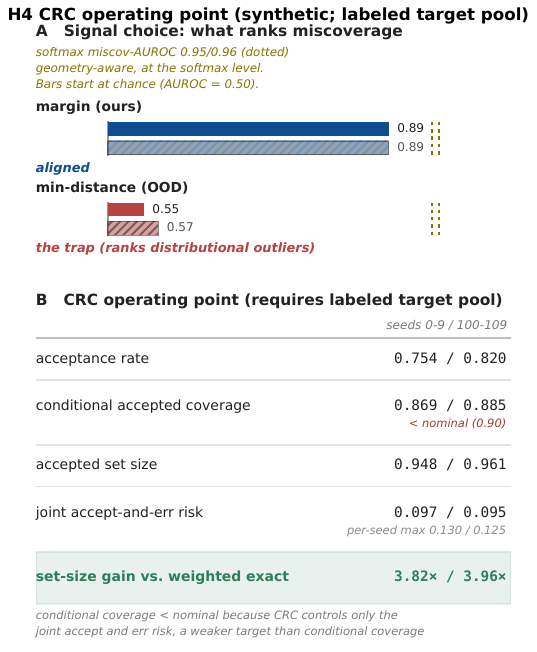}
\caption{\textbf{Synthetic study. H4: signal diagnostics and CRC operating point} (seeds $0$--$9$ / $100$--$109$). CRC threshold calibrated on a \emph{labeled target pool}; not deployable without target labels. Synthetic setting: $K{=}5$, $d{=}6$, shift $0.3$.}
\label{fig:h4crc}
\end{figure}

\begin{figure}[tbp]
\centering
\includegraphics[width=\linewidth]{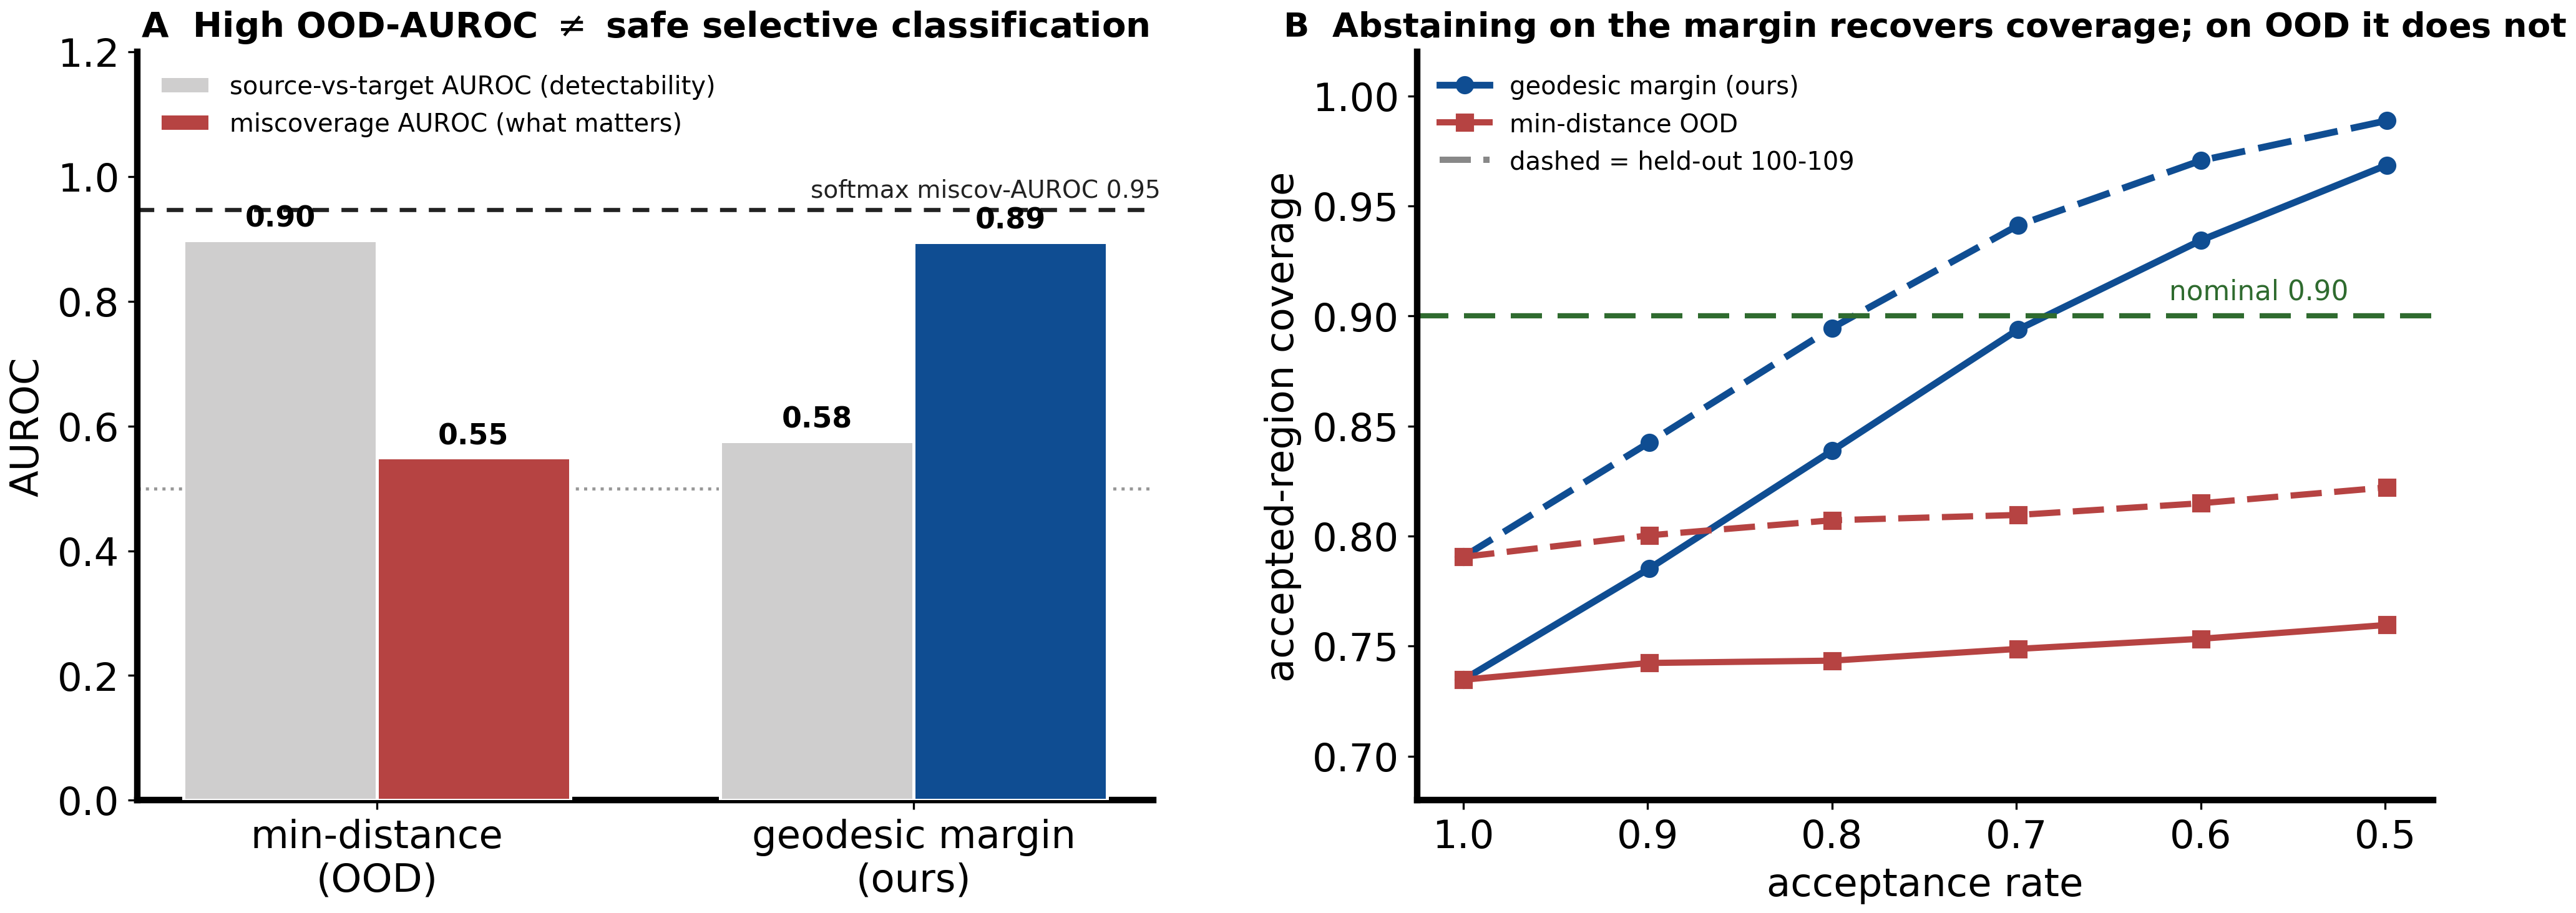}
\caption{\textbf{Synthetic study. The OOD-AUROC trap.} (A) Min-distance: high OOD-AUROC, low
miscoverage AUROC. Geodesic margin: reverse. (B) Abstaining on margin (blue) raises accepted
coverage; abstaining on min distance (red) stays below nominal. Note: ``past nominal'' here refers
only to a test label selected frontier, an oracle diagnostic that is not deployable; the CRC
point itself gives $0.869/0.885 < $ nominal.
Solid $=$ seeds $0$--$9$, dashed $=$ $100$--$109$. Synthetic setting: $K{=}5$, shift $0.3$.}
\label{fig:dichotomy}
\end{figure}

\begin{figure}[tbp]
\centering
\includegraphics[width=\linewidth]{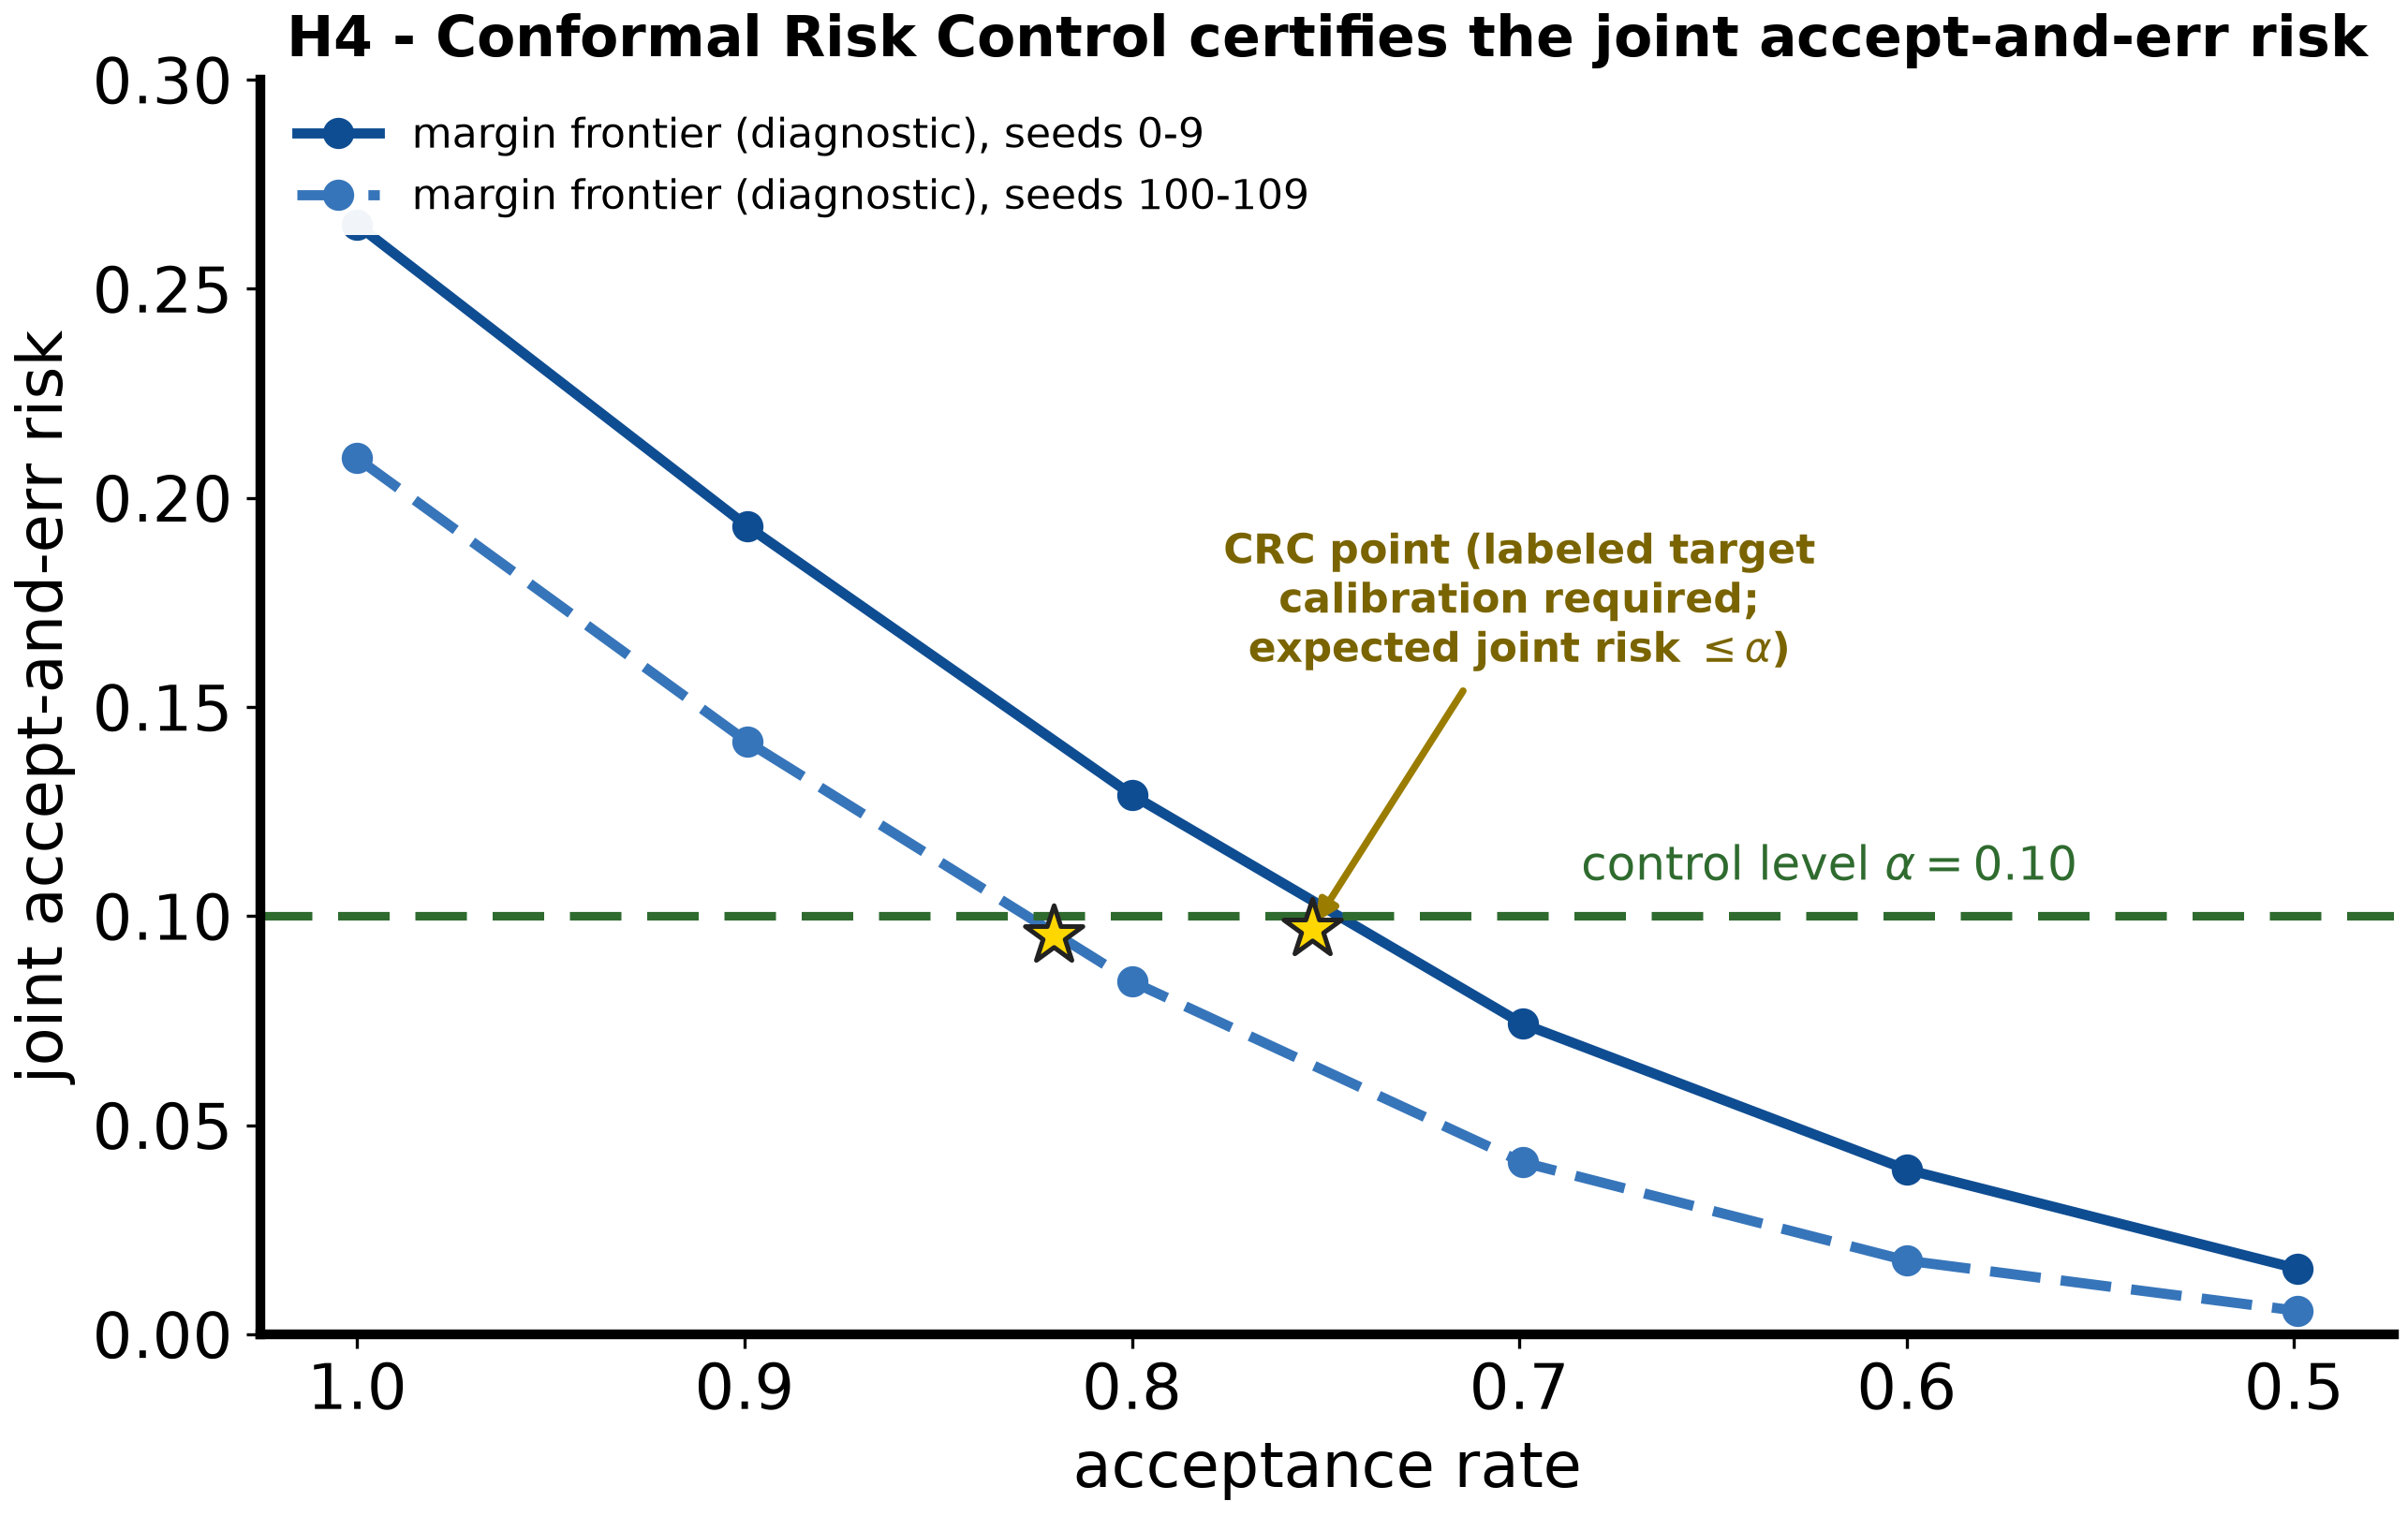}
\caption{\textbf{Synthetic study. CRC certifies the joint risk.} Joint accept and err risk along the
margin frontier vs.\ acceptance rate; CRC operating point (stars) at $\alpha{=}0.10$ control line.
Threshold calibrated on labeled target pool. Synthetic setting: $K{=}5$, shift $0.3$.}
\label{fig:crc}
\end{figure}

\begin{figure}[tbp]
\centering
\includegraphics[width=\linewidth]{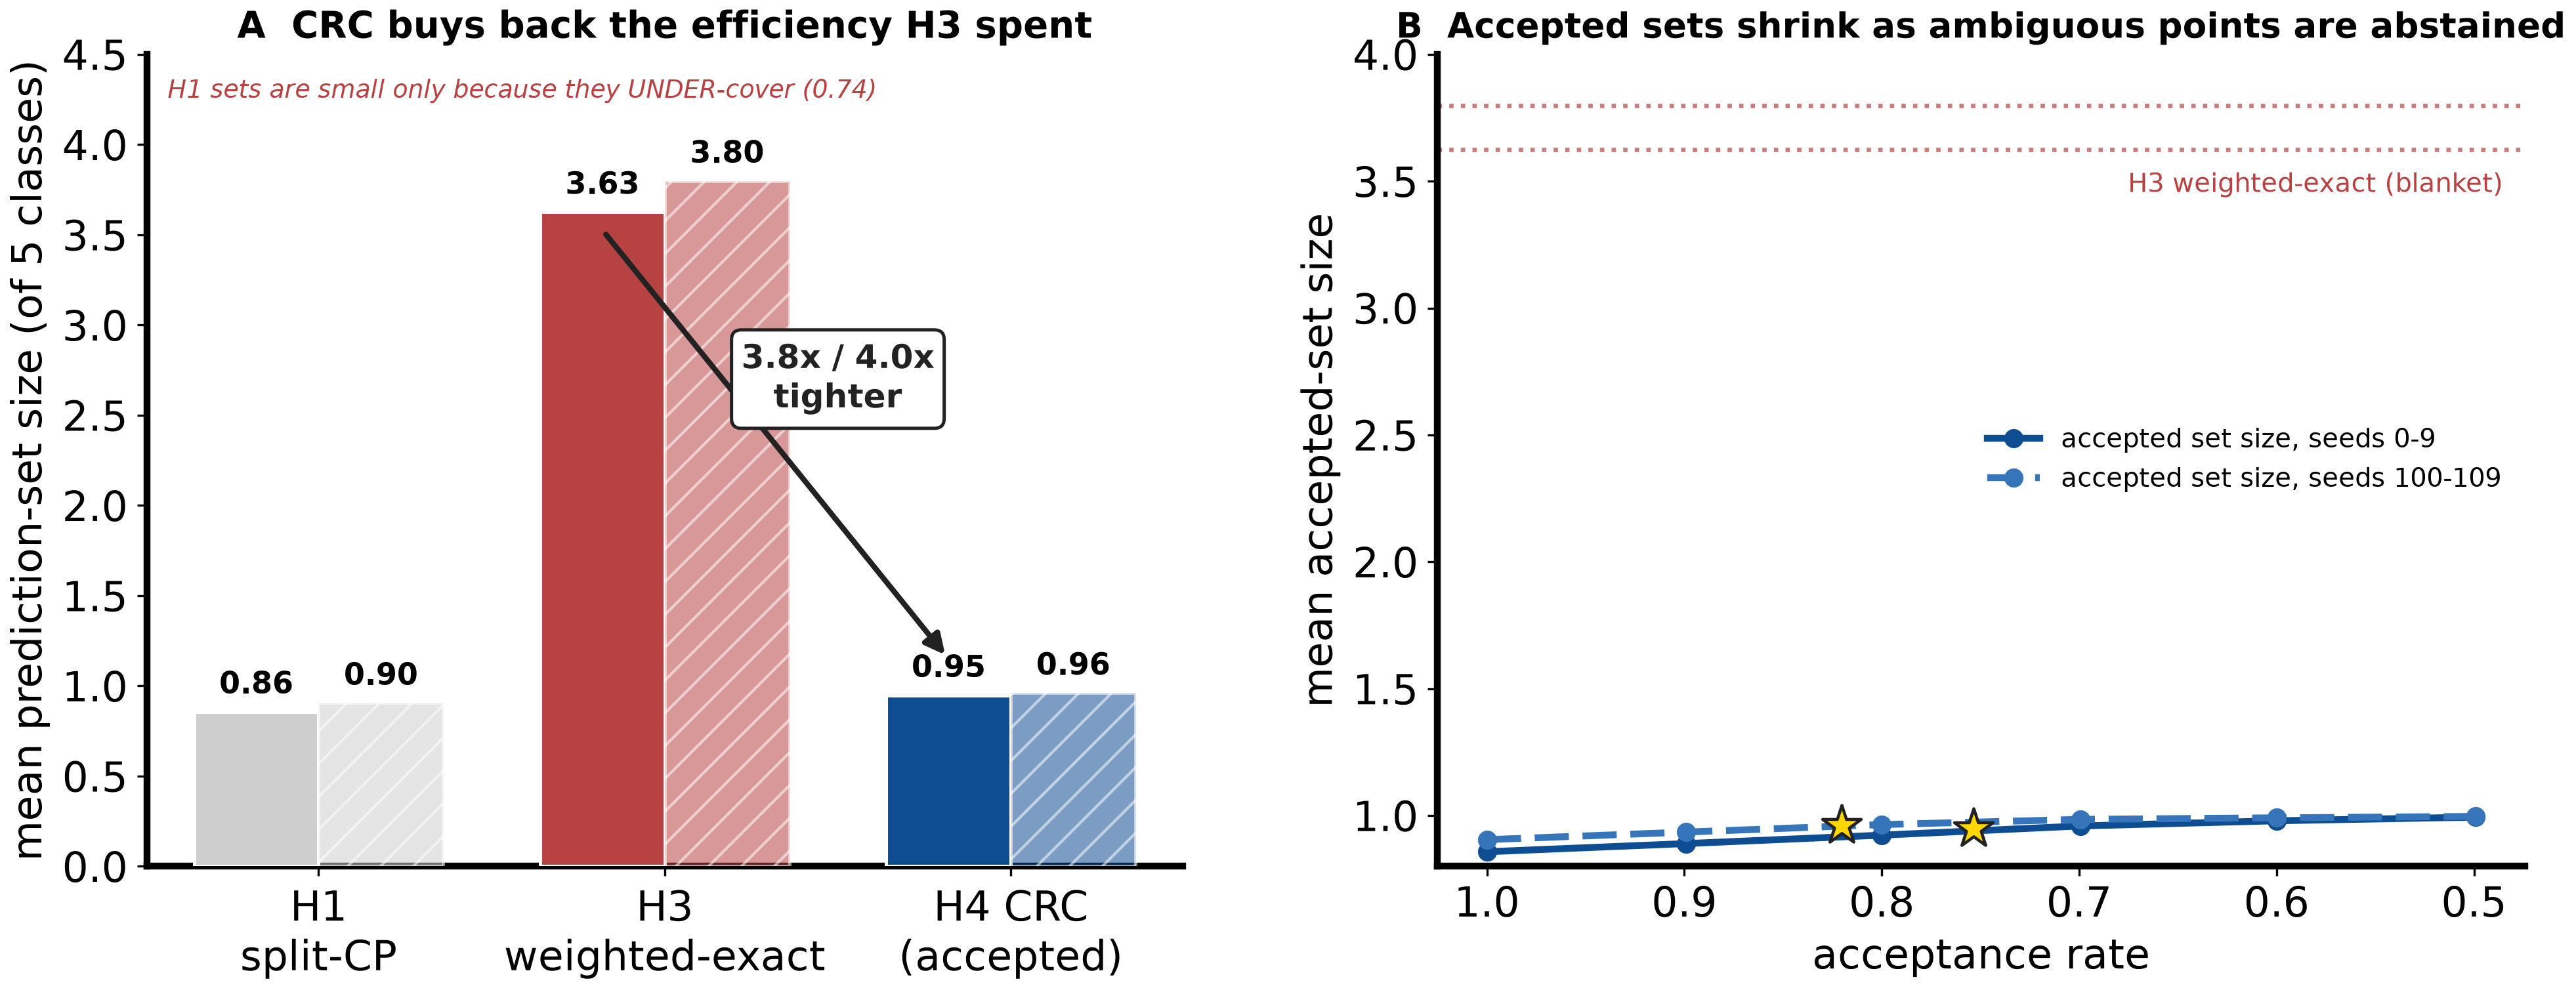}
\caption{\textbf{Synthetic study. Accepted set size vs.\ acceptance rate.} (A) The CRC operating point
achieves $3.82\times/3.96\times$ smaller accepted sets than weighted exact, at the cost of
abstaining on $24.6\%/18.0\%$ of points (acceptance $0.754/0.820$). (B) Accepted set size along the margin frontier; the CRC
point (star) is far below weighted exact's blanket size (dotted).
Synthetic setting: $K{=}5$, shift $0.3$.}
\label{fig:efficiency}
\end{figure}
 
\clearpage  %
\bibliographystyle{apalike}
\bibliography{refs}

\end{document}
